# Supplementary material for: The Rate-Distortion-Perception Trade-off with Side Information
Source: arXiv:2305.13116 source file (2023-05-22)
Supplement: Supplementary file 1 [file removed_section_markov_chains.tex]

\subsubsection{Markov chains}
\hfill\\
The following results will be used during mutual information computations.

\begin{proposition}\label{prop:Markov_property_X_Z}
Let $A,B,C,D$ be subsets of $[n]$ such that\\ $A \subseteq B$ and $C \subseteq [n] \backslash A.$ Then
$$Z_A \independent (J,M,X_C) | X_B, Z_D.$$
\end{proposition} In particular $D$ can be empty. 
\begin{IEEEproof}
Since $P$ is induced by a code we have $J \independent (X^n, Z^n)$ and $Z^n \independent M | J, X^n.$ These imply inequalities between Shannon quantities with respect to $P$ as follows:
\begin{IEEEeqnarray}{rCl}
    \IEEEeqnarraymulticol{3}{l}{I(Z_A; M, J, X_C | X_B, Z_D)\nonumber} \\*
    &=& I(Z_A; J| X_B, Z_D) + I(Z_A; M, X_C | J, X_B, Z_D) \nonumber \\*
    &\leq& I(Z_A, X_B, Z_D; J) + I(Z_A; M, X_{[n]\backslash A} | J, X_B, Z_D) \nonumber \\*
    &\leq& 0 + I(Z_A; X_{[n]\backslash A} | J, X_B, Z_D) + I(Z_A; M | J, X_B, X_{[n]\backslash A}, Z_D) \nonumber \\*
    &\leq& I(Z_A, Z_{D\cap A}, X_B; X_{[n]\backslash A}, Z_{D \cap ([n] \backslash A)} | J) \nonumber \\*
    &+& I(Z_A, Z_D; M | J, X^n) \nonumber \\*
    &=& 0. \nonumber
\end{IEEEeqnarray}
\end{IEEEproof}
Further similar conditional independence relations can be derived using the following lemma:

\begin{lemma}\label{lemma:basic_weak_union}
    For random variables $K,L,W$ we have $$W \independent (K,L) \implies W \independent K | L \text{ and } W \independent K. $$
\end{lemma}

\begin{proposition}\label{prop:Markov_property_Y_X}
Let $A,B,C,D$ be subsets of $[n]$ such that\\ $[n] \backslash A \subseteq B$ and $D \subseteq A.$ Then
$$Y_C \independent X_D | M, J, Z_A, X_B.$$
\end{proposition} In particular $C$ can be equal to $[n].$

\begin{IEEEproof}
We have the following inequalities between Shannon quantities with respect to $P:$
\begin{IEEEeqnarray}{rCl}
    \IEEEeqnarraymulticol{3}{l}{I(Y_C; X_D | M, J, Z_A, X_B)\nonumber} \\*
    &\leq& I(Y^n, Z_{[n] \backslash A}; X_D | M, J, Z_A, X_B) \nonumber \\*
    &\leq& I(Z_{[n] \backslash A}; X_D | M, J, Z_A, X_B) \nonumber \\*
    &+& I(Y^n; X_D | M, J, Z^n, X_B) \nonumber \\*
    &\leq& I(Z_{[n] \backslash A}; X_D | M, J, Z_A, X_B) \nonumber \\*
    &+& I(Y^n; X_D, X_B | M, J, Z^n). \nonumber
\end{IEEEeqnarray} Since $[n] \backslash A \subseteq B$ and $D \subseteq A = [n] \backslash ([n] \backslash A)$ the first term is null by Proposition \ref{prop:Markov_property_X_Z} and Lemma \ref{lemma:basic_weak_union}. Since $P$ is induced by a code we have $Y^n \independent X^n | M, J, Z^n$ and therefore the second term is also null.
\end{IEEEproof}

\begin{lemma}\label{lemma:from_t_to_T__X_Z}
Let $(W(t))_{1\leq t \leq n}$ be a family of random variables such that $\forall t, T \independent (X_t, Z_t, W(t)).$ Then \begin{IEEEeqnarray}{rCl}
    I(W(T), T; X_T|Z_T) &=& I(W(T); X_T|Z_T, T) \nonumber \\*
    &=& \dfrac{1}{n} \sum_{t=1}^n I(W(t); X_t | Z_t). \nonumber
\end{IEEEeqnarray}
\end{lemma}
Proposition \ref{prop:Markov_property_X_Z} and Lemmas \ref{lemma:basic_weak_union}, \ref{lemma:from_t_to_T__X_Z} imply the following:
\begin{corollary}\label{lemma:Markov_chain_X_T_Z_T}
Let $(B(t))_{1\leq t \leq n},(C(t))_{1\leq t \leq n}$ be families of subsets of $[n]$ such that for all $t \in [n]$ we have $t \notin B(t)$ and $t \notin C(t).$ Then
$$Z_T \independent (M, J, T, X_{B(T)}, Z_{C(T)}) | X_T.$$
\end{corollary} In particular, one can choose $B(t) = t+1:n,$ and $C(t) = 1:t-1.$

\begin{lemma}\label{lemma:from_t_to_T__Y_X}
Let $(W(t))_{1\leq t \leq n}$ be a family of random variables such that $\forall t, T \independent (W(t), Z(t)).$ Then \begin{IEEEeqnarray}{rCl}
    I(Y_T; X_T|W(T), Z_T, T) &=& \dfrac{1}{n} \sum_{t=1}^n I(Y_t; X_t | W(t), Z_t). \nonumber
\end{IEEEeqnarray}
\end{lemma}

\noindent Proposition \ref{prop:Markov_property_Y_X} and Lemma \ref{lemma:from_t_to_T__Y_X} imply the following:
\begin{corollary}\label{lemma:Markov_chain_Y_T_X_T}
Let $(B(t))_{1\leq t \leq n},(C(t))_{1\leq t \leq n}$ be families of subsets of $[n]$ such that for all $t \in [n]$ we have $t \notin B(t),$ $t \notin C(t)$ and $[n] \backslash C(t) \subseteq \{t\} \cup B(t).$ Then
$$Y_T \independent X_T | M, J, T, X_{B(T)}, Z_{C(T)}, Z_T.$$
\end{corollary} In particular, one can choose $B(t) = t+1:n,$ and $C(t) = 1:t-1.$\\
