# Supplementary material for: The Rate-Distortion-Perception Trade-off with Side Information
Source: arXiv:2305.13116 source file (2023-05-22)
Supplement: Supplementary file 2 [file removed_showing_likelihood_encoder.tex]

\subsubsection{$P^{(1)}$ is induced by a D-code}
\hfill\\
We fix a positive integer $n.$
Distribution $Q^{(2)}$ satisfies certain Markov properties inherent to its construction. We can then derive the following from \eqref{eq:def_Q_1}, \eqref{eq:def_Q_2} and \eqref{eq:def_P_1}:
\begin{IEEEeqnarray}{rCl}
\IEEEeqnarraymulticol{3}{l}{
P^{(1)} \: (m,m',j,x^n,y^n,z^n, \hat{m}')
}\nonumber\\*
& = & \tfrac{\text{\normalsize 1}}{\lfloor 2^{nR_c} \rfloor} \ \prod_{t=1}^n \raisebox{2pt}{\scalebox{1.1}{$p$}} \substack{\scalebox{1.0}{$ \: (x_t, z_t) $} \\ \scalebox{0.7}{$X, Z \qquad \quad$} } \ \substack{\scalebox{1.0}{$Q^{(2)} \; (m,m') \qquad \qquad $} \\ \scalebox{0.7}{$M, M'| J\text{=}j, X^n\text{=}x^n, Z^n\text{=}z^n$}} \nonumber\\*
% &  & \substack{\scalebox{1.0}{$\mathbf{1} \qquad \qquad \qquad$}  \\ v^n = v^n(m,m',j)} \nonumber\\*
&&\substack{ \raisebox{-2pt}{$P^{D,n}$} \scalebox{1.0}{$ \; (\hat{m}') \qquad \qquad \quad \;$} \\ \hat{M}' | M=m, J=j, Z^n=z^n} \substack{\scalebox{1.0}{$P^{(1)} \; (y^n) \qquad \qquad \qquad $} \\ \scalebox{0.7}{$Y^n| V^n\text{=}v^n(m, \hat{m}', j), Z^n\text{=}z^n$}}. \label{eq:rewrite_P_1}
\end{IEEEeqnarray}
\noindent We can use Markov property $Z-X-V$ from \eqref{eq:def_S_D} to show that $(M,M')$ can be sampled according to $Q^{(2)}$ without relying on $Z^n:$
\begin{IEEEeqnarray}{rCl}
\IEEEeqnarraymulticol{3}{l}{
\substack{\scalebox{1.0}{$Q^{(2)} \; (m,m') \qquad \qquad \qquad  $} \\ \scalebox{0.7}{$M, M'| J\text{=}j, X^n\text{=}x^n, Z^n\text{=}z^n$}}
}\nonumber\\*
&=&\dfrac{Q^{(2)}(m,m',j,x^n,z^n)}{\sum_{\tilde{m}, \tilde{m}'} Q^{(2)}(\tilde{m}, \tilde{m}',j,x^n,z^n)}\nonumber\\*
&=&\dfrac{Q^{(2)}(m,m',j,x^n) \ \raisebox{2pt}{\scalebox{1.1}{$p$}} \substack{\scalebox{1.0}{$ \: (z_t) $} \\ \scalebox{0.7}{$Z^n | X^n\text{=}x^n, V^n\text{=}v^n(m, m', j)$} }}{\sum_{\tilde{m}, \tilde{m}'} Q^{(2)}(\tilde{m}, \tilde{m}',j,x^n) \ \raisebox{2pt}{\scalebox{1.1}{$p$}} \substack{\scalebox{1.0}{$ \: (z_t) $} \\ \scalebox{0.7}{$Z^n | X^n\text{=}x^n, V^n\text{=}v^n(\tilde{m}, \tilde{m}', j)$} }}\nonumber\\*
&=&\dfrac{Q^{(2)}(m,m',j,x^n) \ \raisebox{2pt}{\scalebox{1.1}{$p$}} \substack{\scalebox{1.0}{$ \: (z_t) $} \\ \scalebox{0.7}{$Z^n | X^n\text{=}x^n$} }}{\sum_{\tilde{m}, \tilde{m}'} Q^{(2)}(\tilde{m}, \tilde{m}',j,x^n) \ \raisebox{2pt}{\scalebox{1.1}{$p$}} \substack{\scalebox{1.0}{$ \: (z_t) $} \\ \scalebox{0.7}{$Z^n | X^n\text{=}x^n$} }}\nonumber\\*
&=& \substack{\scalebox{1.0}{$Q^{(2)} \; (m,m') \qquad \qquad \qquad  $} \\ \scalebox{0.7}{$M, M'| J\text{=}j, X^n\text{=}x^n$}}. \label{eq:likelihood_encoder}\IEEEeqnarraynumspace
\end{IEEEeqnarray}
Finally, for every positive integer $n$ our coding scheme is as follows:
\begin{itemize}
    \item Both the encoder and decoder have access to codebook $c_*^{(n)}.$
    \item The encoder uses its inputs $x^n$ and $j$ to sample a message $m$ using $Q^{(2)}_{M|\mathcal{C}^{(n)}\text{=}c_*^{(n)}, J\text{=}j, X^n\text{=}x^n}.$
    \item The decoder uses $m$ and its inputs $z^n$ and $j$ to decode the virtual message $\hat{m}'$ using $P^{D,n}.$
    \item Finally the decoder uses $z^n$ and codeword $v^n(c_*^{(n)}, m, \hat{m}', j)$ to sample and output a sequence $y^n$ via $Q^{(2)}_{Y^n| V^n\text{=}v^n(c_*^{(n)}, m, \hat{m}', j), Z^n\text{=}z^n}.$
\end{itemize}
By construction of $\mathcal{C}^{(n)}$ the codebook $c_*^{(n)}$ is adapted to message rate $R+\varepsilon$ and common randomness rate $R_c.$ By \eqref{eq:rewrite_P_1} and \eqref{eq:likelihood_encoder} the variables in this scheme have joint distribution equal to $P^{(1)}.$\\
