# Supplementary material for: The Rate-Distortion-Perception Trade-off with Side Information
Source: arXiv:2305.13116 source file (2023-05-22)
Supplement: Supplementary file 3 [file main_file_appendix.tex]

\newpage
%%%%%% 
%% Appendix:
%% If needed a single appendix is created by
%%
\appendix
%%
%% If several appendices are needed, then the command
%%
%\appendices
%%
%% in combination with further \section-commands can be used.
%%%%%%

The appendix (or appendices) are optional. For reviewing purposes,
additional 5~pages (double-column) are allowed (resulting in a maximum
grand total of 10~pages plus one page containing only
references). These additional 5~pages must be removed in the final
version of an accepted paper.

\subsection{Measure-theoretic justifications}
\subsubsection{General results}\label{app:measure_theory_general}
\hfill\\
%\todo[inline]{Say that we define conditional distributions of $p$ knowing null density values by using the dominating distribution, e.g. $p(x|v) = \mu$ if $?(v)=0.$ Need to fix a density $?$ to be able to talk about "the values $v$ for which $?(v)=0.$" and say once and for all that a consequence is that all distributions defined subsequently will similarly defined everywhere. And the latter and all densities are UNIQUELY defined.}
%\todo[inline]{Also clarify that any conditional distrib of $X^n, Y^n$ is w.r.t $\mu^n$ }
\todo[inline]{I think that uniform integrability does not depend on the underlying probability space as long as it is a standard probability space. If time, look at the commented todonote in Section \ref{app:info_theory_for_general_spaces}}
\todo[inline]{Check no assumption of existence of a density anywhere, unless it is $P<<P+Q$}
\todo[inline]{Fix quads and qquads in distributions}
A measurable space on a discrete alphabet will always be endowed with its power set $\sigma$-algebra and a product of the two measurable spaces will be implicitly endowed with the product $\sigma$-algebra. A conditional probability kernel is defined for all elements of the input alphabet (not just a.e.):
\begin{definition}
    Given any two measurable spaces $(\mathcal{W}, \mathcal{B})$ and $(\mathcal{W}', \mathcal{B}'),$ a \textit{regular channel}, also called a \textit{regular conditional or transition probability kernel} from the former to the latter is a function from $\mathcal{W}\times \mathcal{B}'$ to $[0,1]$ such that $\forall w \in \mathcal{W}, \rho(w,\cdot)$ is a probability distribution on $(\mathcal{W}', \mathcal{B}')$ and $\forall B' \in \mathcal{B}',$ $\rho(\cdot, B')$ is $\mathcal{B}$-measurable. The kernel is said to be \textit{dominated} by a $\sigma$-finite measure $\mu$ on $(\mathcal{W}', \mathcal{B}')$ if for every $w \in \mathcal{W},$ $\rho(w,\cdot)$ is. We then write $\rho \ll \mu.$
\end{definition}
\vspace{5pt}
% We follow standard practice in probability theory regarding product spaces and transition probabilities.
% Throughout this paper we implicitly rely on the following facts (see e.g. \cite{1995ProbabilityAndMeasure}). The domination of any joint distribution by a product $\sigma$-finite measures ensures the existence of conditional densities and probability kernels -this would also be true if one only assumed that the spaces are Polish. For every conditional probability considered we implicitly assume that one such kernel has been chosen. Moreover, domination and $\sigma$-finiteness are inherited in sequential definitions: for any joint distribution defined by a marginal and a transition kernel which are respectively dominated by two $\sigma$-finite measures, the joint distribution is dominated by the product measure and the latter is $\sigma$-finite.\\

We define measures sequentially by defining regular transition probabilities. This is well defined and grants the generalized Fubini theorem (see, e.g. \cite{1995ProbabilityAndMeasure}):
\begin{theorem}(Generalized Fubini theorem)\\
Consider any two measurable spaces $(\mathcal{W}, \mathcal{B})$ and $(\mathcal{W}', \mathcal{B}'),$ a probability measure $\mu$ on the former and a transition kernel $\rho(\cdot, \cdot)$ from $(\mathcal{W}, \mathcal{B})$ to $(\mathcal{W}', \mathcal{B}').$ Then there is a unique measure $Q$ on the product space $(\mathcal{W}\times\mathcal{W}', \mathcal{B}\otimes\mathcal{B}')$ with\begin{equation*}
    \forall B\in \mathcal{B}, \forall B' \in \mathcal{B}', \ Q(B\times B') = \int_B \rho(B',w) d\mu(w).
\end{equation*} Moreover, for any non-negative measurable function $\varphi,$ we have\begin{equation*}
    \int \varphi \ dQ = \int \bigg(\int \varphi \ d\rho(w, \cdot) \bigg) d\mu(w).
\end{equation*}
\end{theorem}
When given a joint distribution, such as from $\mathcal{D}_D,$ we extensively use corresponding conditional distributions, which is justified if the alphabets are Polish spaces accoring to the following theorem, sometimes referred to as Jirina's theorem.
\begin{theorem}\cite[Theorem~9.2.2]{BookWithJirinaTheorem2010}\label{theorem:jirina}
Let $\mathcal{W}$ and $\mathcal{W}'$ be Polish spaces and $\Omega=\mathcal{W}\times \mathcal{W}',$ endowed with their respective Borel $\sigma$-algebras. Let $Q$ be a probability measure on $\Omega,$ with marginal on $\mathcal{W}$ denoted by $\mu.$ Then, there exists a probability transition kernel $\rho(\cdot, \cdot)$ from $\mathcal{W}$ to $\mathcal{W}'$ such that for any non-negative measurable function $\varphi,$ we have\begin{equation*}
    \int \varphi \ dQ = \int \bigg(\int \varphi \ d\rho(w, \cdot) \bigg) d\mu(w).
\end{equation*}
Moreover, for any measurable set $B'\subset \mathcal{W}',$ the measurable map $w \mapsto \rho(w, B')$ is unique up to a $\mu$-null set.
\end{theorem}
\vspace{5pt}
The family of Polish spaces includes all discrete spaces and real vector spaces $\mathbb{R}^k,$ and any finite product of Polish spaces is a Polish space.

\subsubsection{Total variation distance for general alphabets}\label{app:TV_lemmas_for_general_alphabets}
\hfill\\
\todo[inline]{If time add a proof of Lemma \ref{lemma:TV_due_to_M_and_hatM}}
It is well known that the total variation distance between distributions $P,Q,$ defined by $\sup_{A}\{P(A)\text{-}Q(A)\},$ is equal to \begin{equation}
   \dfrac{1}{2} \int |p-q|d\mu = \int (p-q)^{+}d\mu,
\end{equation} for any common dominating $\mu$ and corresponding densities $p,q.$
We now prove Lemma \ref{lemma:get_expectation_out_of_TV}, \ref{lemma:TV_joint_to_TV_marginal} and \ref{lemma:TV_same_channel} in this order.
\begin{IEEEproof}
Fix a probability measure $\mu$ dominating both $\Pi_W \Pi_{L|W}$ and $\Pi_W \Gamma_{L|W}$ -e.g. ($\Pi_W \Pi_{L|W}+\Pi_W \Gamma_{L|W})/2$ - and denote the respective densities by $\pi$ and $\gamma.$ Since the alphabets are Polish, then by Theorem \ref{theorem:jirina}, measure $\mu$ admits a regular conditional probability kernel and satisfies the generalized Fubini property. Therefore, both laws have marginal $\Pi_W$ with density with respect to marginal $\mu_W$ given by \begin{equation*}
    \pi(w)=\gamma(w) = \int \pi(w,l) d\mu_{L|W=w}(l).
\end{equation*} Moreover, the transition kernels defined on $\{\pi(W)>0\}$ by \begin{equation*}
    \pi(w,\cdot)/\pi(w) \cdot \mu_{L|W=w}, \quad \gamma(w,l)/\gamma(w) \cdot \mu_{L|W=w}
\end{equation*}and some fixed distribution on $\{\pi(W)=0\}$ are regular and satisfy the generalized Fubini property because $\mu$ does. By the uniqueness result in Theorem \ref{theorem:jirina}, these kernels yield the same integrals on $\mathcal{W}\times \mathcal{L}$ as $\Pi_{L|W}$ and $\Gamma_{L|W}.$ The result is obtained by choosing $\varphi= (w,l)\mapsto|\pi(w,l)-\gamma(w,l)|$ in Theorem \ref{theorem:jirina}.
\end{IEEEproof}

\begin{IEEEproof}
    \begin{equation*}
        \sup_{A \subset \mathcal{W}\times\mathcal{L}}\{P(A)\text{-}Q(A)\} \geq \sup_{B \subset \mathcal{W}}\{P(B\times\mathcal{L})\text{-}Q(B\times\mathcal{L})\}.
    \end{equation*}
\end{IEEEproof}

\begin{IEEEproof}
    $\Pi$ and $\Gamma$ are dominated by the probability measure $\mu$ defined with marginal $\mu_W=(\Pi_W + \Gamma_W)/2$ and channel $\Pi_{L|W},$ and their densities are $d\Pi_W/d\mu_W$ and $d\Gamma_W/d\mu_W.$
\end{IEEEproof}

\subsection{Treatment of distributions on products of discrete and continuous alphabets}

\subsubsection{Fundamental definitions and results}\label{app:info_theory_for_general_spaces}
\hfill\\
We use the following results from \cite{Wyner1978GeneralConditionalMutualInformation} and references therein. Mutual information is well-defined for general random variables without any assumption on the underlying probability space by the two equivalent definitions.
\begin{definition}\label{def:KL_mutual_info}
Let $(X,Y)$ be a couple of joint distribution $P_{X,Y}.$ Product distribution $P_X\otimes P_Y$ is then dominated by $p_{X,Y}$ and we denote its density by $p.$ We define\begin{equation}
    I(X;Y) = \int p(x,y)\log(p(x,v))dP_{X,Y}(x,y),
\end{equation}where the negative part of the integrand is integrable. The integrand is then integrable iff $I(X;Y)<\infty.$ The term $\log(p(x,v))$ is often denoted $i(x,y).$
\end{definition}
\begin{theorem}
    \begin{equation}
        I(X;Y) = \sup_{[X], [Y]} I([X];[Y]),
    \end{equation}where $[X]$ (resp. $[Y]$) denotes any image of $X$ (resp. $Y$) by a finite-valued map.
\end{theorem}
Moreover, for the mutual information of two tuples, the supremum can be restricted to quantizations of each coordinate, ie rectangular quantization grids. Conditional mutual information is defined similarly, as well as the conditional entropy of a discrete variable conditioned on general variables. All properties of mutual information from the discrete case generalize as long as no entropy of an infinite-valued variable is used, nor any substraction of mutual information terms.
\subsubsection{Form of the soft covering lemma for mixed variables}\label{app:sup_mutual_info}
\hfill\\
The result \cite[Corollary~VII.4]{2013PaulCuffDistributedChannelSynthesis} is stated with the spectral sup-mutual information:\begin{equation*}
    \overline{I}(Z;V) = \inf\{\tau: p_{Z,V}^{\otimes n} \big( (1/n) i(Z^n,V^n) > \tau\big) \to 0\},
\end{equation*}where $i$ is as in Definition \ref{def:KL_mutual_info}. But we know that $I_p(Z;V)$ is finite, which implies that $i\log(i)$ is integrable and hence the law of large numbers applies. Therefore, by additivity of $i$ for product distributions, the spectral sup-mutual information is the mutual information.

\subsubsection{Decoder for $M'$ in the case of infinite alphabets}\label{app:decoder_M_prime}
\hfill\\
By definition of $R',$ if $I_p(Z;V)=0$ then $R'=0$ and the alphabet of $M'$ is a singleton, and therefore $M'$ can be decoded perfectly for any choice of decoder. Suppose the contrary. Then, by definition of $R'$ we have $R'<I_p(Z;V).$ 
%Moreover, if each of $\mathcal{Z}$ and $\mathcal{V}$ is finite then by the standard result for discrete memoryless channels (see e.g. \cite{Cover&Thomas2006}), the decoding error can be made to vanish as stated in Section \ref{sec:Q_1}. Suppose the contrary. Then Lemma \ref{lemma:cells_with_arbitrarily_low_probability} applies: there exists a a positive integer $\kappa$ such that in the regular quantization grid of $\mathcal{Z}\times \mathcal{V}$ of parameter $\kappa,$ the $p_{Z,V}$-probability of every cell is less that $2^{-3n(R+R'+R_c)}.$ 
Since $R'<I_p(Z;V),$ then from the results mentioned in Section \ref{app:info_theory_for_general_spaces} that there exists a quantized tuple $([Z], [V])$ such that $I_p([Z]; [V]) > R'.$ 
%and having a quantization grid that is more refined than the regular grid of parameter $\kappa.$ In particular, it is such that $[V] \equiv V$ if $\mathcal{V}$ is finite. 
As depicted in Figure \ref{fig:quantization_setup}, we extend the definition of $Q^{(1)}$ from \eqref{eq:def_Q_1} by:
\begin{figure}[t!]
    \centering\includegraphics[width=0.48\textwidth]{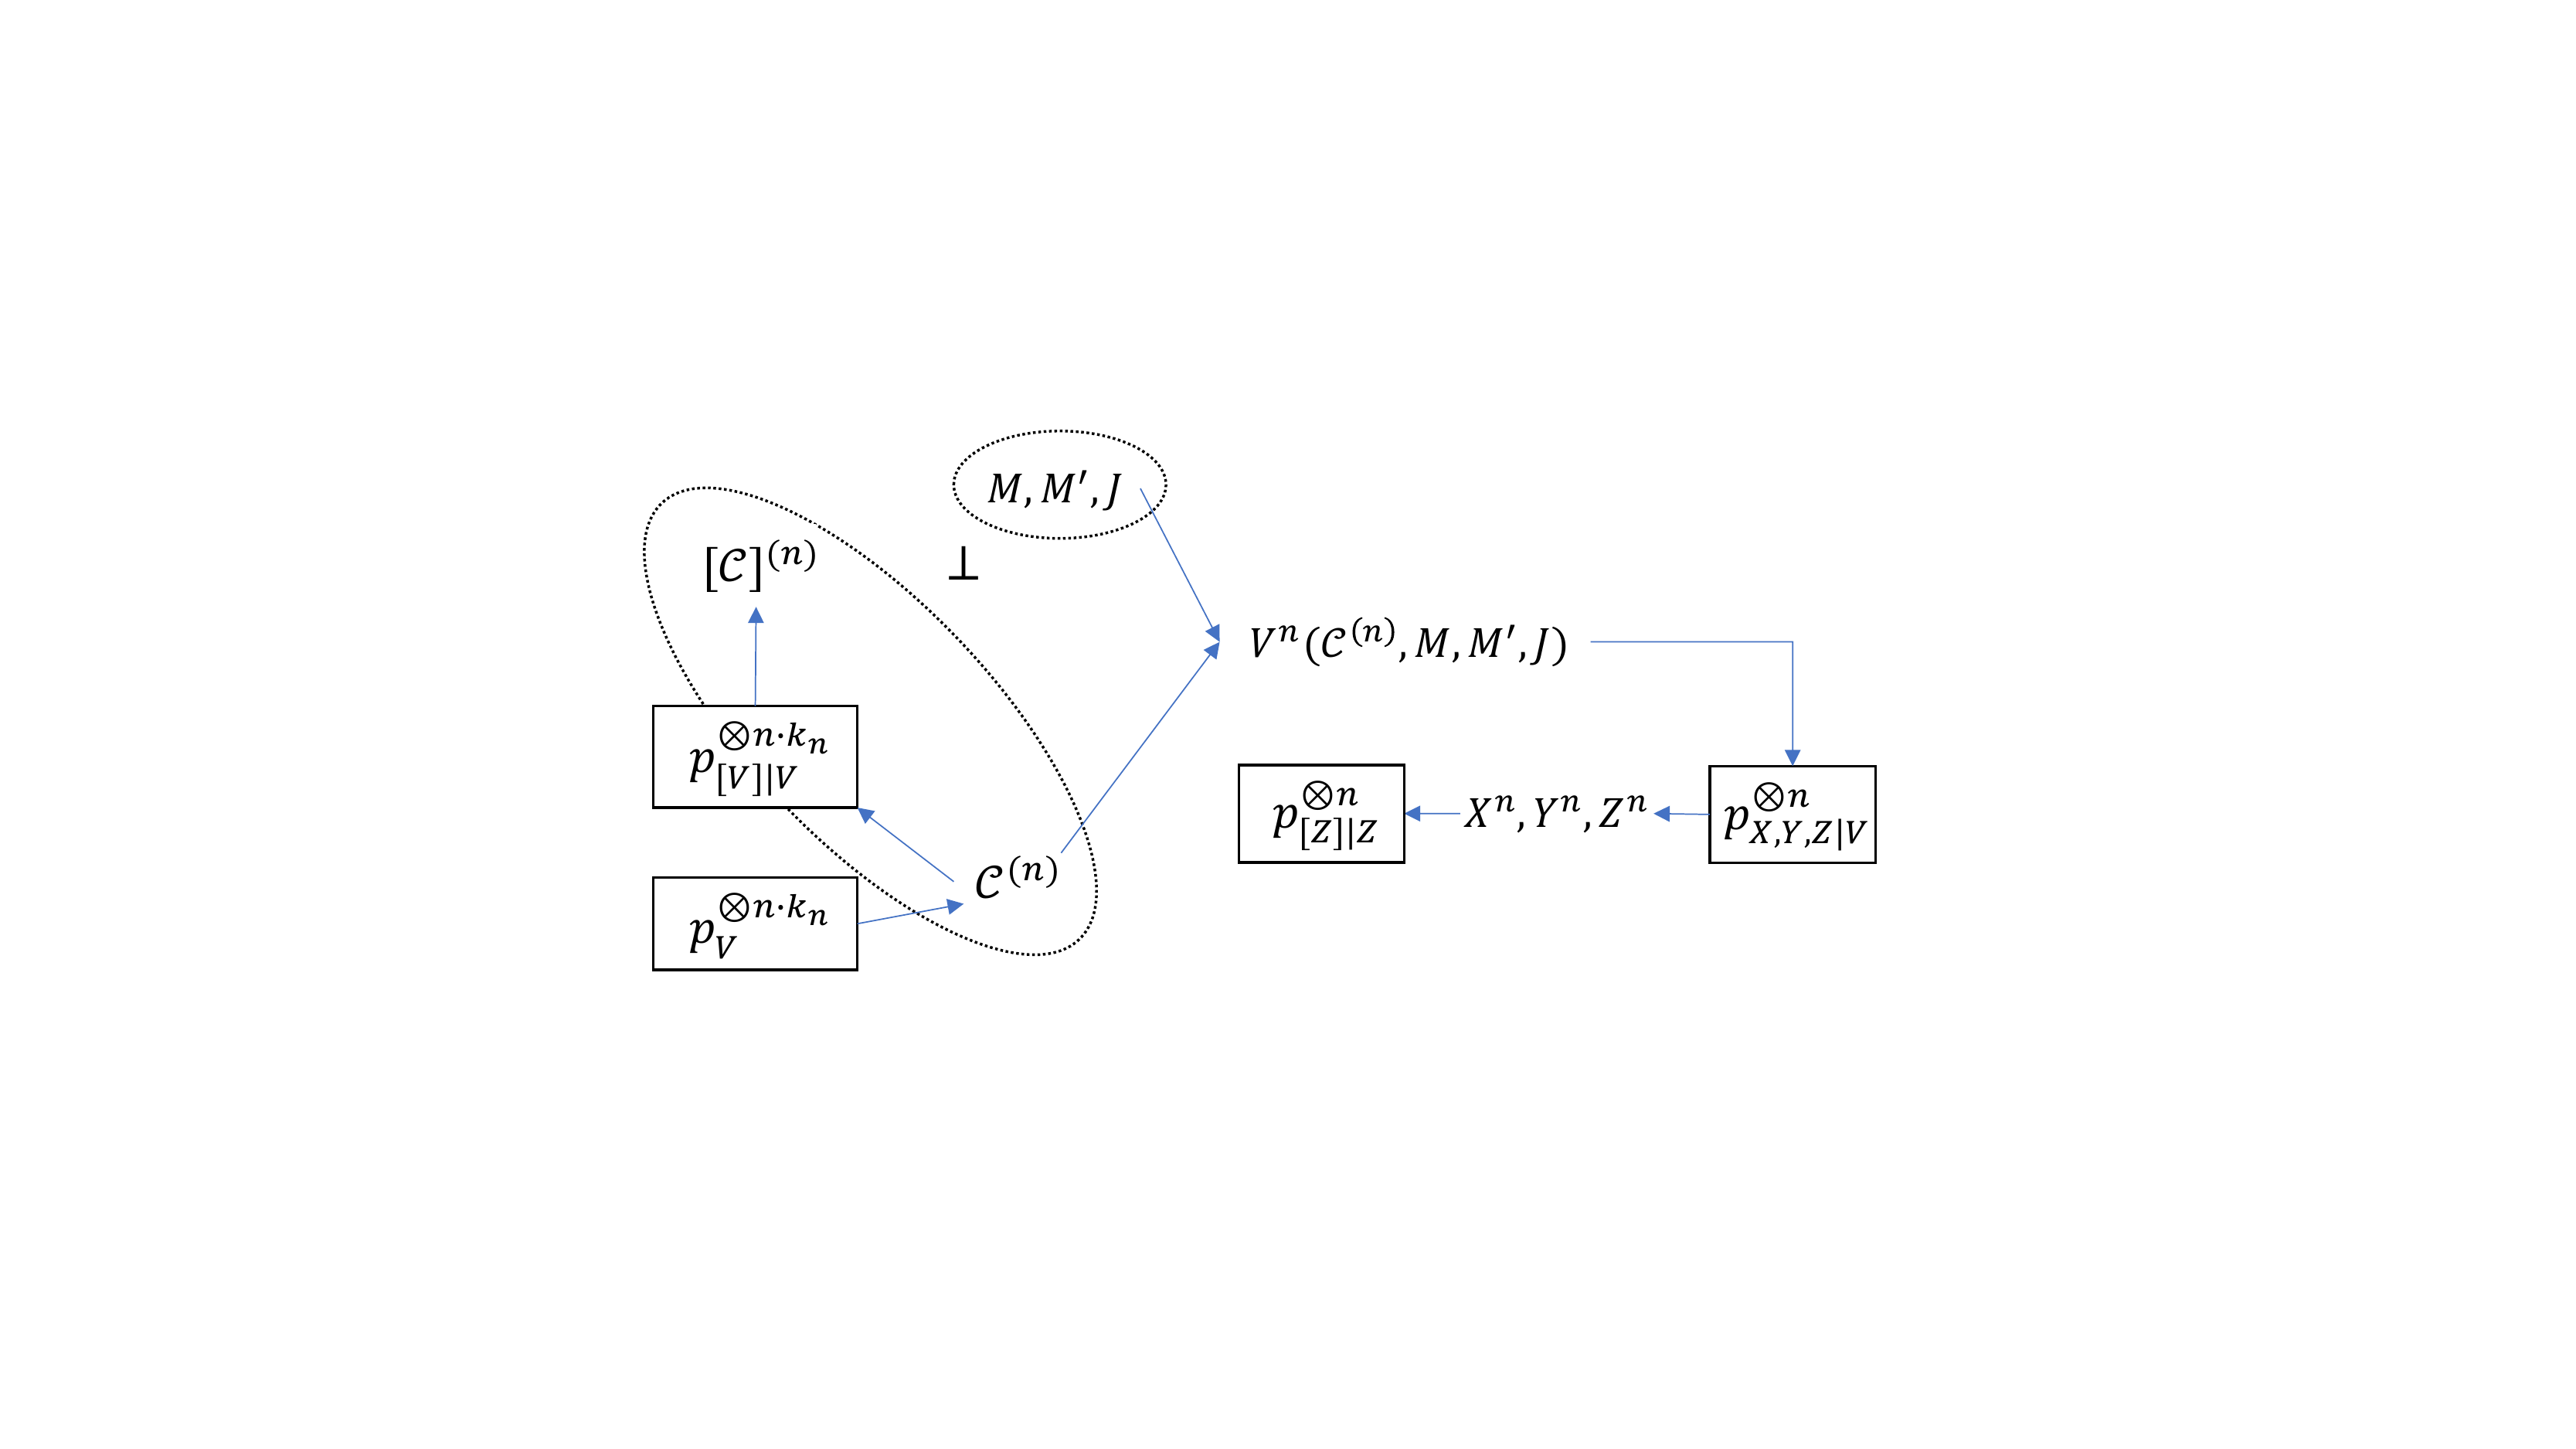}
    \caption{Graphical model for $Q^{(1)}$ with quantized variables, where $k_n = \lfloor 2^{n(R+\varepsilon)}\rfloor \times \lfloor 2^{nR'}\rfloor \times \lfloor 2^{nR_c}\rfloor.$ The variables inside a dashed oval are independent from variables inside another oval.}
    \label{fig:quantization_setup}
\end{figure}
\begin{equation}\label{eq:def_single_letter_quantization}
    p_{V,X,Y,Z,[V],[Z]} = p_{V,X,Y,Z}\cdot p_{[V]|V} \cdot p_{[Z]|Z} \text{ and}
\end{equation}\begin{IEEEeqnarray}{rCl}
\IEEEeqnarraymulticol{3}{l}{
\substack{\scalebox{1.0}{$Q^{(1)} \; ([c]^{(n)}, [z]^n, \hat{m}') \qquad \qquad \qquad \qquad \qquad \qquad \qquad \quad \;$} \\ [\mathcal{C}]^{(n)}, [Z]^n, \hat{M}' |\mathcal{C}^{(n)}\text{=}c^{(n)}, M\text{=}m, M'\text{=}m', J\text{=}j, X^n\text{=}x^n, Y^n\text{=}y^n, Z^n\text{=}z^n}
}\nonumber\\*
\quad & = & \prod_{k=1}^n \raisebox{2pt}{\scalebox{1.1}{$p$}} \substack{\scalebox{1.0}{$ \: ([z]_k)$} \\ \scalebox{0.7}{$[Z]|Z\text{=}z_k$} } \prod_{j,m,m'} \prod_{k=1}^n \raisebox{2pt}{\scalebox{1.1}{$p$}} \substack{\scalebox{1.0}{$ ([v]_k) \qquad \qquad $} \\ \scalebox{0.7}{$[V]|V\text{=}v_k(c^{(n)}, m, m', j)$} }\nonumber\\*
&& \substack{ \raisebox{-2pt}{$P^{D}$} \scalebox{1.0}{$ \; (\hat{m}') \qquad \qquad \qquad \qquad \qquad \; \ $} \\ \hat{M}' | [\mathcal{C}]^{(n)}=[c]^{(n)}, M=m, J=j, [Z]^n=[z]^n}, \label{eq:def_quantized_codebook_and_P_D}
\end{IEEEeqnarray}where $P^D$ represents, for each $(m,j),$ the joint typicality decoder of \cite{Cover&Thomas2006} for the joint distribution $p_{[V],[Z]}$ and codebook $(V^n([\mathcal{C}]^{(n)}, m, a, j))_a.$ We check that this setting is that of the channel random coding proof of \cite{Cover&Thomas2006}. Similarly to $\mathcal{C}^{(n)},$ we denote the codewords in $[\mathcal{C}]^{(n)}$ by $[V]^n([\mathcal{C}]^{(n)}, m, m', j).$\\ 

Fix a couple $(m,j).$ By the above definition \eqref{eq:def_quantized_codebook_and_P_D}, the definition of $\mathbb{Q}_{\mathcal{C}^{(n)}},$ and the independence (see \eqref{eq:def_Q_1}) of $\mathcal{C}^{(n)}$ and $(M,J)$ under $Q^{(1)},$ then knowing $M=m, J=j$ the random codebook $(V^n([\mathcal{C}]^{(n)}, j,m,a))_a$ consists of $\lfloor 2^{nR'}\rfloor$ i.i.d. codewords sampled from $p_{[V]}^{\otimes n}.$
Moreover, when conditioning on $([\mathcal{C}]^{(n)}, M,M',J)=([c]^{(n)}, m,m',j),$ as can be seen from the graphical model in Figure \ref{fig:quantization_setup} or from equations \eqref{eq:def_Q_1} and \eqref{eq:def_quantized_codebook_and_P_D}, the distribution of $[Z^n]$ is that of the output of the $n$-fold product of the discrete memoryless channel $p_{V|[V]} \cdot p_{Z|V} \cdot p_{[Z]|Z},$ with input $[v]^n([c]^{(n)}, m, m', j).$ Therefore, the proof in \cite{Cover&Thomas2006} applies: since by assumption the codebook rate satisfies $0<R'<I_p([V]; [Z]),$ we have
\begin{IEEEeqnarray}{c}
\substack{\scalebox{1.0}{$Q^{(1)} \; (\hat{M}'\neq \ M') $} \\ \hat{M}', M' |M=m, J=j } \underset{n \to \infty}{\longrightarrow} 0. \label{eq:Q_1_decoding_error_fixed_sub_codebook_general_sources} \IEEEeqnarraynumspace
\end{IEEEeqnarray}
%defining, for every $n \geq 1$ and every $(m,j) \in [2^{n(R+\varepsilon)}] \times [2^{nR_c}],$ $\Tilde{P}^{D,n}_{\hat{M}'|M, J, Z^n, \mathcal{C}^{(n)}}$ to be the joint typicality decoder applied after quantization of $Z^n,$ we get $P(\hat{M}' \neq [V^n(\mathcal{C}^n, j,m,M')]).$ Then, if $V$ is finite then by assumption the quantization is the identity map.
Since nothing in this proof depends on the particular value $(m,j),$ including the sub-codebook's distribution, the conditional distribution in \eqref{eq:Q_1_decoding_error_fixed_sub_codebook_general_sources} does not depend on $(m,j).$Hence
\begin{IEEEeqnarray}{c}
\substack{\scalebox{1.0}{$Q^{(1)} \; (\hat{M}'\neq \ M') $} \\ \hat{M}', M' \qquad \qquad} \underset{n \to \infty}{\longrightarrow} 0. \label{eq:Q_1_decoding_error_fixed_codebook_general_sources} \IEEEeqnarraynumspace
\end{IEEEeqnarray}

\todo[inline]{Replace $P_{X|Y=y}(x)$ by $P_{X|Y}(x|y)$ everywhere}
\todo[inline]{Check that no Greek letter is used for two concepts.}

\subsection{Further justifications}
\subsubsection{Equivalence between achievability with near-perfect and perfect realism}\label{app:equivalence_perfect_realism}
\hfill\\
In order to prove Theorem \ref{theorem:equivalence_perfect_realism}, we state the following result, which corresponds to Remark \ref{remark:existence_of_prop_to_perfect_realism} and which we also use in Section \ref{sec:achievability}.
\begin{proposition}\label{proposition:to_perfect_realism}
Let $n$ be a positive integer and $\varepsilon_1, \varepsilon_2, \varepsilon_3$ be positive reals. Let $\mathcal{X}$ and $\mathcal{Z}$ be two Polish alphabets and $p_{X,Z}$ be a joint distribution on $\mathcal{X} \times \mathcal{Z}.$ 
%dominated by a product of $\sigma$-finite measures $\mu$ and $\gamma.$ 
Let $d$ be a distortion measure such that $(d,p_X)$ is uniformly integrable. Let $Q_{X^n, Y^n}$ be a distribution on $\mathcal{X}^n \times \mathcal{X}^n$ satisfying
\begin{IEEEeqnarray}{rCl}
\IEEEeqnarraymulticol{3}{l}{
\mathbb{E}_Q[d(X^n, Y^n)] \leq \Delta + \varepsilon_1 
} \label{eq:distortion_assumption_theorem_to_perfect_realism}\\*
&\text{ and } \| Q_{Y^n} - p_X^{\otimes n} \|_{TV} \leq \varepsilon_2.& \label{eq:perception_assumption_theorem_to_perfect_realism}
\end{IEEEeqnarray} Let $P^{(1)}$ be a distribution induced (Definition \ref{def:achievability}) by a $(n,R,R_c)$ D-code (resp. E-D-code) for some reals $R,R_c\geq 0.$ Assume that \begin{equation}
    \| P^{(1)}_{X^n, Y^n} - Q_{X^n, Y^n} \|_{TV} \leq \varepsilon_3.\label{eq:total_variation_Q_P_assumption_theorem_to_perfect_realism}
\end{equation} Then there is a $(n,R,R_c)$ D-code (resp. E-D-code) with the same encoder as $P^{(1)}$ and inducing a distribution $P^{(2)}$ with
\begin{IEEEeqnarray}{rCl}
\IEEEeqnarraymulticol{3}{l}{
\mathbb{E}_{P^{(2)}}[d(X^n, Y^n)] \leq \Delta + \varepsilon_1 + \sup_{X,Y,B}\mathbb{E}[d(X, Y) \ \scalebox{1.0}{$\mathbf{1}_B $}]
} \label{eq:distortion_result_theorem_to_perfect_realism}\\*
&\text{ and } P^{(2)}_{Y^n} \equiv p_X^{\otimes n},& \label{eq:perception_result_theorem_to_perfect_realism}
\end{IEEEeqnarray} where the supremum is over all variables $X$ and $Y$ having law $p_X$ and all events $B$ with probability at most $\varepsilon_2 + 2\varepsilon_3.$
\end{proposition}
\vspace{5pt}
%We start by showing how 
Proposition \ref{proposition:to_perfect_realism} implies Theorem \ref{theorem:equivalence_perfect_realism} by taking $Q\equiv P^{(1)}$ at fixed blocklength.
% \begin{IEEEproof}
% We know that the D(resp. E-D)-achievability with perfect realism implies that with near-perfect realism. Consider a triplet $(R,R_c,\Delta)$ D(resp. E-D)-achievable with near-perfect realism and a corresponding sequence of $(n, R, R_c)$ codes $(F^{(n)},G^{(n)})_n.$ 
% %and two vanishing sequences $(\varepsilon_{1,n})_n, (\varepsilon_{2,n})_n$ of positive reals such that for every $n,$
% %\begin{IEEEeqnarray}{rCl}
% %\IEEEeqnarraymulticol{3}{l}{
% %\mathbb{E}_{P^{(n)}}[d(X^n, Y^n)] \leq \Delta + \varepsilon_{1,n} 
% %} \\*
% %\text{ and } \| P^{(n)}_{Y^n} - p_X^{\otimes n} \|_{TV} \leq %\varepsilon_{2,n}.&& 
% %\end{IEEEeqnarray}
% Then the achievability with perfect realism is obtained by using Proposition \ref{proposition:to_perfect_realism} with the $Q\equiv P^{(1)}$ and equal to the distribution induced by the $n$-th code, and by the uniform integrability assumption.
% %$\varepsilon_1=\varepsilon_{1,n}, \varepsilon_2=\varepsilon_{2,n}, \varepsilon_3=0,$ there exists a sequence of codes and their corresponding distributions $(\Tilde{P}^{(n)})_n$ such that for all $n$
% % \begin{IEEEeqnarray}{rCl}
% % \IEEEeqnarraymulticol{3}{l}{
% % \mathbb{E}_{\Tilde{P}^{(n)}}[d(X^n, Y^n)] \leq \Delta + \varepsilon_{1,n} + \varepsilon_{2,n}
% % } \label{eq:distortion_result_theorem_to_perfect_realism}\\*
% % &\text{ and } \Tilde{P}^{(n)}_{Y^n} \equiv p_X^{\otimes n}.& \label{eq:perception_result_theorem_to_perfect_realism}
% % \end{IEEEeqnarray}
% \end{IEEEproof}
%We now prove Proposition \ref{proposition:to_perfect_realism} and divide the proof in two parts.\\
We prove Proposition \ref{proposition:to_perfect_realism} in the next two subsections.
\subsubsection{Modified code satisfying perfect realism}
\hfill\\
Consider the setting of Proposition \eqref{proposition:to_perfect_realism}. If $P^{(1)}_{Y^n} \equiv p_{X}^{\otimes n},$ we just set $P^{(2)} \equiv P^{(1)}.$ Assume this is not the case.
By Definition \ref{def:achievability}, the conditional distribution of $Y^n$ knowing all other variables reduces to $P^{(1)}_{Y^n|Z^n,M,J}.$ Let $\mu$ be $\sigma$-finite and dominating $P^{(1)}_{Y^n}$ and $p_{X}^{\otimes n},$ e.g. $P^{(1)}_{Y^n} + p_{X}^{\otimes n}.$ Let
\begin{IEEEeqnarray}{c}
    \mathcal{X}^n_{+} = \bigg\{ y^n \in \mathcal{X}^n \text{s.t.} \dfrac{dP^{(1)}_{Y^n}}{d\mu}(y^n) > \dfrac{dp_{X}^{\otimes n}}{d\mu}(y^n) \bigg\} \nonumber\\*
    \text{and } \theta_n: \mathcal{X}^n_{+} \to \mathbb{R}, y^n \mapsto \dfrac{dp_{X}^{\otimes n}/d\mu(y^n)}{dP^{(1)}_{Y^n}/d\mu(y^n)}.\nonumber
\end{IEEEeqnarray}
For any $z^n, m, j$ and any set $A \in \mathcal{X}^n$ we define
\begin{IEEEeqnarray}{rCl}
\IEEEeqnarraymulticol{3}{l}{
P^{(2)}(A |z^n, m, j) = P^{(1)}(A \backslash \mathcal{X}^n_{+} |z^n, m, j) \ +
}\nonumber\\*
& & \int_{A \cap \mathcal{X}^n_{+}} \theta_n(y^n) dP^{(1)}(y^n|z^n, m, j) + \phi_{z^n, m, j} \Gamma(A) \text{ where} \nonumber\\*
&&\Gamma(A) = \dfrac{\int_A (dp_{X}^{\otimes n}/d\mu(y^n) - dP^{(1)}_{Y^n}/d\mu(y^n))^{+} d\mu(y^n)}{\int (dp_{X}^{\otimes n}/d\mu(y^n) - dP^{(1)}_{Y^n}/d\mu(y^n))^{+} d\mu(y^n)}\nonumber\\*
&& \text{and } \phi_{z^n, m, j} = \int_{\mathcal{X}^n_{+}} 1 - \theta^n(y^n) dP^{(1)}(y^n|z^n, m, j). \label{eq:def_phi_bis}
\end{IEEEeqnarray}
It can be checked that this defines a probability measure for every $z^n, m, j.$ 
%The first two terms are non-negative measures because defined from non-negative density functions with respect to $P^{(1)}_{Y^n|Z^n, M, J}.$ The same applies to the third term defined with respect to $\mu,$ with the non-negativity of constant $\phi_{z^n, m, j}$ coming from the fact that by definition we have $\theta^n < 1$ on $\mathcal{X}^n_{+}.$ Finally we have $\Gamma(\mathcal{X}^n)=1,$ giving $P^{(2)}(\mathcal{X}^n|z^n, m, j) = 1.$ 
We define the joint distribution for the new code as
\begin{equation}\label{eq:def_P_2_bis}
    P^{(2)}_{\scalebox{0.7}{$X^n, Z^n, M, J, Y^n$}} = P^{(1)}_{\scalebox{0.7}{$X^n, Z^n, M, J$}}P^{(2)}_{\scalebox{0.7}{$Y^n| Z^n, M, J$}}.
\end{equation}
% \begin{IEEEeqnarray}{rCl}
% \IEEEeqnarraymulticol{3}{l}{
% P^{(2)}(\mathcal{X}^n|z^n, m, j) = P^{(1)}(\mathcal{X}^n \backslash \mathcal{X}^n_{+} |z^n, m, j) \ +
% }\nonumber\\*
% & & \int_{ \mathcal{X}^n_{+}} \theta_n(y^n) dP^{(1)}(y^n|z^n, m, j) + \int_{\mathcal{X}^n_{+}} 1 - \theta^n(y^n) dP^{(1)}(y^n|z^n, m, j) \nonumber\\*
% &&\nonumber\\*
% && . \nonumber\end{IEEEeqnarray}
Then similarly to $P^{(1)},$ $P^{(2)}$ is the distribution induced by a $(n,R,R_c)$ D(resp. E-D)-code. Moreover the latter has the same encoder as $P^{(1)}.$ Based on this and since the definition of $P^{(2)}(\cdot | z^n, m, j)$ is affine in $P^{(1)}(\cdot | z^n, m, j),$ one can show that $P^{(2)}$ satisfies perfect realism by taking the expectation according to $P^{(1)}_{Z^n, M, J}$ and using Fubini's theorem for non-negative variables.
% \begin{IEEEeqnarray}{rCl}
% P^{(2)}_{Y^n}(A) &=& P^{(1)}_{Y^n}(A \backslash \mathcal{X}^n_{+}) \ + \int_{A \cap \mathcal{X}^n_{+}} \theta_n(y^n) dP^{(1)}_{Y^n}(y^n) \nonumber\\*
% & + &  \Gamma(A) \int_{\mathcal{X}^n_{+}} 1 - \theta^n(y^n) dP^{(1)}_{Y^n}(y^n) \nonumber\\*
% &=& P^{(1)}_{Y^n}(A \backslash \mathcal{X}^n_{+}) \ + p_{X}^{\otimes n}(A \cap \mathcal{X}^n_{+})  \nonumber\\*
% & + &  \Gamma(A) \int_{\mathcal{X}^n_{+}} \tfrac{dP^{(1)}_{Y^n}}{d\mu}(y^n) - \tfrac{dp_{X}^{\otimes n}}{d\mu}(y^n) d\mu(y^n) \nonumber.
% \end{IEEEeqnarray} By definition of $\mathcal{X}^n_{+},$ the last term reduces to the numerator of $\Gamma(A),$ which reduces to 
% \begin{IEEEeqnarray}{rCl}
% \IEEEeqnarraymulticol{3}{l}{
% \int_{A \backslash \mathcal{X}^n_{+}} \tfrac{dp_{X}^{\otimes n}}{d\mu}(y^n) - \tfrac{dP^{(1)}_{Y^n}}{d\mu}(y^n) d\mu(y^n)
% }\nonumber\\*
% & = & p_{X}^{\otimes n}(A \backslash \mathcal{X}^n_{+}) - P^{(1)}_{Y^n}(A \backslash \mathcal{X}^n_{+}). \nonumber
% \end{IEEEeqnarray}
The last step consists in obtaining the distortion bound by coupling $P^{(2)}$ with $Q.$\\
\subsubsection{Coupling with $Q$}
\hfill\\
We first compare $P^{(2)}$ to $P^{(1)}.$ For every $z^n, m, j$ and every set $A \in \mathcal{X}^n$ we have:
\begin{IEEEeqnarray}{rCl}
\IEEEeqnarraymulticol{3}{l}{
P^{(1)}(A |z^n, m, j) - P^{(2)}(A |z^n, m, j)
}\nonumber\\*
& = & \int_{A \cap \mathcal{X}^n_{+}} 1 - \theta_n(y^n) dP^{(1)}(y^n|z^n, m, j) - \phi_{z^n, m, j} \Gamma(A). \nonumber
\end{IEEEeqnarray} Both terms being smaller than or equal to $\phi_{z^n, m, j},$ we have
\begin{IEEEeqnarray}{c}
    \big\|P^{(2)}_{Y^n|Z^n\text{=}z^n, M\text{=}m, J\text{=}j} - P^{(1)}_{Y^n|Z^n\text{=}z^n, M\text{=}m, J\text{=}j}\big\|_{TV} \leq \phi_{z^n, m, j}.\nonumber
\end{IEEEeqnarray}
When integrating this over all variables except $Y^n,$ we get by definition \eqref{eq:def_P_2_bis} of $P^{(2)}$ and Lemma \ref{lemma:get_expectation_out_of_TV} on the one hand and by definition \eqref{eq:def_phi_bis} of $\phi$ and Fubini's theorem on the other hand:
\begin{IEEEeqnarray}{rCl}
\IEEEeqnarraymulticol{3}{l}{
\big\|P^{(2)}_{\scalebox{0.6}{$X^n, Z^n, M, J, Y^n$}} - P^{(1)}_{\scalebox{0.6}{$X^n, Z^n, M, J, Y^n$}}\big\|_{TV}
}\nonumber\\*
%& \leq & \int \phi_{z^n, m, j} dP^{(1)}_{\scalebox{0.6}{$X^n, Z^n, M, J$}} \nonumber\\*
&\leq& \int_{\mathcal{X}^n_{+}} 1 - \theta^n(y^n) dP^{(1)}_{Y^n}(y^n) = \big\|P^{(1)}_{Y^n} - p_{X}^{\otimes n} \big\|_{TV}.\nonumber
\end{IEEEeqnarray}
Therefore by Lemma \ref{lemma:TV_joint_to_TV_marginal} applied to assumption \eqref{eq:total_variation_Q_P_assumption_theorem_to_perfect_realism} with $W=Y^n$ and by the triangle inequality and assumption \eqref{eq:perception_assumption_theorem_to_perfect_realism} we get
\begin{IEEEeqnarray}{c}
    \big\|P^{(2)}_{\scalebox{0.6}{$X^n, Z^n, M, J, Y^n$}} - P^{(1)}_{\scalebox{0.6}{$X^n, Z^n, M, J, Y^n$}}\big\|_{TV} \leq \varepsilon_2 + \varepsilon_3.\nonumber
\end{IEEEeqnarray}
Therefore by Lemma \ref{lemma:TV_joint_to_TV_marginal} with $W=(X^n, Y^n)$ and $W=Y^n$ and the triangle inequality with assumption \eqref{eq:total_variation_Q_P_assumption_theorem_to_perfect_realism} we get
\begin{IEEEeqnarray}{c}
    \big\|P^{(2)}_{X^n,Y^n} - Q_{X^n,Y^n}\big\|_{TV} \leq \varepsilon_2 + 2\varepsilon_3. \IEEEeqnarraynumspace \label{eq:TV_on_X_and_Y_P_2_Q_anonymous}
\end{IEEEeqnarray}
We then use the following standard coupling lemma (see e.g. \cite[Chapter~I, Theorem~5.2]{1992Coupling_Book}):
% \begin{lemma}\label{lemma:coupling_existence_bis}
% For any two probability measures $\Pi, \Pi'$ on a measurable space there exists a probability measure $\rho$ and a random tuple $(W,W')$ with distribution $\rho$ with marginals $\rho_W \equiv \Pi$ and $\rho_{W'} \equiv \Pi'$ and such that $\rho(W \neq W') = \|\Pi - \Pi'\|_{TV}.$
% \end{lemma}
%Thus 
by \eqref{eq:TV_on_X_and_Y_P_2_Q_anonymous} there exists a quadruple $(X^n, Y^n, \Tilde{X}^n, \Tilde{Y}^n)$ with distribution denoted by $\rho$ having marginals $P^{(2)}_{X^n,Y^n}$ and $Q_{X^n,Y^n}$ and such that $\rho((X^n, Y^n)\neq (\Tilde{X}^n, \Tilde{Y}^n)) \leq \varepsilon_2 + 2\varepsilon_3.$ We then have
\begin{IEEEeqnarray}{rCl}
\IEEEeqnarraymulticol{3}{l}{
\mathbb{E}_{P^{(2)}}[d(X^n, Y^n)] = \mathbb{E}_{\rho}[d(X^n, Y^n)]
}\nonumber\\*
&=& \mathbb{E}_{\rho}\Big[d(\Tilde{X}^n, \Tilde{Y}^n)\substack{\scalebox{1.0}{$\mathbf{1} \qquad \qquad \qquad \quad$}  \\ (X^n, Y^n) = (\Tilde{X}^n, \Tilde{Y}^n)}\Big] \nonumber \\*
&+& \mathbb{E}_{\rho}\Big[d(X^n, Y^n)\substack{\scalebox{1.0}{$\mathbf{1} \qquad \qquad \qquad \quad$}  \\ (X^n, Y^n) \neq (\Tilde{X}^n, \Tilde{Y}^n)}\Big] \nonumber\\*
&\leq& \mathbb{E}_{Q}[d(X^n, Y^n)] + \tfrac{1}{n}\sum_{i=1}^n \mathbb{E}_{\rho}\Big[d(X_i, Y_i)\substack{\scalebox{1.0}{$\mathbf{1} \qquad \qquad \qquad \quad$}  \\ (X^n, Y^n) \neq (\Tilde{X}^n, \Tilde{Y}^n)}\Big]\nonumber\\*
&\leq& \mathbb{E}_{Q}[d(X^n, Y^n)] + \tfrac{1}{n}\sum_{i=1}^n \sup_{X,Y,B}\mathbb{E}\Big[d(X, Y) \ \scalebox{1.0}{$\mathbf{1}_B $}\Big], \nonumber
\end{IEEEeqnarray} the supremum is over all variables $X$ and $Y$ having law $p_X$ and all events $B$ with $\rho(B) \leq \varepsilon_2 + 2\varepsilon_3,$ and the last inequality holds because $P^{(2)}$ satisfies perfect realism $P^{(2)}_{Y^n} = p_X^{\otimes n}$ and by \eqref{eq:def_P_2_bis} we have $P^{(2)}_{X^n} = p_X^{\otimes n}.$ We conclude by assumption \eqref{eq:distortion_assumption_theorem_to_perfect_realism}.

\subsubsection{Proof of Corollary \ref{corollary:E_D_rates_region}}\label{app:proof_corollary}
\hfill\\
Consider the setting of the corollary. Let $(X,Z)$ be a couple with distribution $p_{X,Z}$ and let $\Tilde{\mathcal{X}} = \mathcal{X} \times \mathcal{Z},$ $\Tilde{\mathcal{Z}} = \mathcal{Z},$ $\Tilde{X} = (X,Z),$ $\Tilde{Z} = Z$ and $\Tilde{p}_{\Tilde{X}, \Tilde{Z}}.$ Define \begin{equation*}
\Tilde{d}: \Tilde{\mathcal{X}} \times \Tilde{\mathcal{X}} \to [0,\infty), \quad (x,z,x',z') \mapsto d(x,x')   
\end{equation*} These new objects statisfy the conditions of Theorem \ref{theorem:D_rates_region}: $(\Tilde{d}, \Tilde{p}_{\Tilde{X}})$ is uniformly integrable because $(d, p_X)$ is. Denote by $\Tilde{\mathcal{S}}_{D,\infty}$ the corresponding region. By Theorem \ref{theorem:equivalence_perfect_realism}, D(resp. E-D)-achievability with near perfect realism is equivalent to D(resp. E-D)-achievability with perfect realism. The latter notion will be used hereafter. Given a D-code for $(\Tilde{d}, \Tilde{p}_{\Tilde{X}, \Tilde{Z}}),$ applying the projection $\pi: (x,z) \mapsto (x',z')$ after the decoder gives a E-D-code for $(d,p_{X,Z}).$ Hence, by Lemma \ref{lemma:TV_joint_to_TV_marginal}, a D-achievable couple $(R,\Delta)$ for $(\Tilde{d}, \Tilde{p}_{\Tilde{X}, \Tilde{Z}})$ is also E-D-achievable for $(d,p_{X,Z}).$ Moreover, given a E-D-achievable couple $(R,\Delta)$ for $(d,p_{X,Z})$ and a corresponding sequence of E-D-codes $(F_n, G_n),$ modifying the decoder to $G^{(n)}_{Y^n|Z^n, J, M} \cdot \prod_{k=1}^n p_{Z|X=Y_k}$ gives a sequences of codes attesting the D-achievability of $(R,\Delta)$ for $(\Tilde{d}, \Tilde{p}_{\Tilde{X}, \Tilde{Z}}).$ Hence Corollary \ref{corollary:E_D_rates_region} holds with $\mathcal{S}_{E\text{-}D,\infty} = \Tilde{\mathcal{S}}_{D,\infty}:$
\begin{align}\label{eq:def_S_E_D_infty_bis}
      & 
    \left\{ \begin{array}{rcl}
        (R, \Delta) \in \mathbb{R}_{\geq 0}^2 &:& \exists \ \Tilde{p}_{X,Z,\Tilde{V},\hat{X}, \hat{Z}} \in \Tilde{D}_D \text{ s.t. } \\
        R &\geq& I_{\Tilde{p}}(\Tilde{V};X|Z) \\
        \Delta &\geq& \mathbb{E}_{\Tilde{p}}[d(X, \hat{X})]
    \end{array}\right\}, 
\end{align}
with $\Tilde{D}_D$ being
\begin{align}\label{eq:def_D_E_D_bis}
       & 
    \left\{ \begin{array}{rcl}
        &\Tilde{p}_{X,Z,\Tilde{V},\hat{X}, \hat{Z}} : \scalebox{0.9}{$(X,Z) \sim$ } p_{X,Z}& \\
        &\Tilde{p}_{\hat{X}, \hat{Z}} \equiv p_{X, Z}&\\
        &X - (Z, \Tilde{V}) - (\hat{X}, \hat{Z})& \\
        &I_{\Tilde{p}}(Z;\Tilde{V}) < \infty&
        %\exists \nu \ \sigma\text{-finite s.t. }& p \ll & \mu \times \gamma \times \nu \times \mu
    \end{array}\right\},
\end{align} where $\Tilde{Y}$ has been replaced by $(\hat{X}, \hat{Z}),$ $I(\Tilde{X}; \Tilde{V}|\Tilde{Z}) = (X,Z;\Tilde{V}|Z) = I(X;\Tilde{V}|Z)$ and the Markov chain $\Tilde{Z}-\Tilde{X}-\Tilde{V}$ is trivial and has been omitted. The region $\Tilde{\mathcal{S}}_{D,\infty}$ is unchanged when replacing $\Tilde{\mathcal{D}}_D$ in \eqref{eq:def_S_E_D_infty_bis} by its successive images through the following maps, which preserve $\mathbb{E}_{\Tilde{p}}[d(X, \hat{X})]$ and 
%diminishes 
$I_{\Tilde{p}}(\Tilde{V};X|Z):$ 
%to $I_{\Tilde{p}}(\hat{X};X|Z)$ (data processing inequality):
\begin{equation*}
    \Tilde{p}_{X,Z,\Tilde{V},\hat{X}, \hat{Z}} \mapsto \Tilde{p}_{X,Z,\Tilde{V},\hat{X}} \cdot p_{Z|X=\hat{X}} \mapsto \Tilde{p}_{X,Z,\Tilde{V},\hat{X}} 
    %\mapsto \Tilde{p}_{X,Z,\hat{X}}.
\end{equation*}This results in a map from $\Tilde{\mathcal{D}}_D$ to $\mathcal{D}_{E\text{-}D}.$ Indeed the first map makes the Markov chain in $\Tilde{\mathcal{D}}_D$ equivalent to $X - (Z, V) - \hat{X}$ and the second removes the unused variable $\hat{Z}.$ Then, $\Tilde{V}$ and $\hat{X}$ can be renamed into $V$ and $Y$ respectively.

\subsubsection{Regarding Markov chains in the converse proof}\label{app:Markov_chains_precise_reference_for_converse}
\hfill\\
In \cite[Appendix~F]{2012YassaeeEtAlInteractiveCommunicationsLongVersion},with $r=1, \omega=J,\mathcal{Y}_1=\emptyset,Y_2=Y, X_1=X, X_2=Z,C_1=M,F_1=V$, the same $V$ as in Section \ref{sec:converse} is used and the same Markov chains are proved. This extends to general alphabets since the proof in \cite{2012YassaeeEtAlInteractiveCommunicationsLongVersion} is only based on the chain rule and conditional independence, without any subtractions of mutual information terms.

\subsubsection{Use of the soft covering lemma}\label{app:use_of_soft_covering}

\begin{lemma}\label{lemma:soft_covering}\cite[Corollary~VII.4]{2013PaulCuffDistributedChannelSynthesis} Let $\mathcal{V}$ be an alphabet and $\rho_V$ a distribution on the latter. Let $R$ be a positive real number. Let $(k_n)_{n \geq 1}$ be a sequence of positive integers such that $k_n$ $\substack{\raisebox{-4pt}{$\sim$} \\ \scalebox{0.5}{$n$$\to$$\infty$}}$ $2^{n(R+\varepsilon)}.$ For every positive integer $n$ let $\mathcal{E}^{(n)}$ be a randomly generated collection of $k_n$ mutually independent sequences in $\mathcal{V}^n$ each drawn according to $\rho_V^{\otimes n}.$ The sequences are indexed by some set $\mathcal{I}$ of size $k_n$ and in a realization $e^{(n)}$ of $\mathcal{E}^{(n)}$ the sequence with index $i$ is denoted by $v^n(e^{(n)}, i).$ A memoryless channel $(\rho_{W|V\text{=}v})_{v \in \mathcal{V}}$ induces an output distribution defined as
    $$\text{$\Gamma$}\substack{\; \; \scalebox{0.85}{$(i,v^n,w^n) \qquad $} \\ \scalebox{0.6}{$I, V^n, W^n |\mathcal{E}^{(n)}=e^{(n)}$}}  = \dfrac{1}{k_n} \; \; \substack{\scalebox{1.2}{$\mathbf{1} \qquad \qquad $} \\ v^n = v^n(e^{(n)}, i)} \prod_{t=1}^n \rho \substack{\scalebox{0.8}{$ (w_t) $} \\ \scalebox{0.55}{$W|V=v_t$} } \ .$$
    If $R > I_{\rho}(V;W)$ then
    $$\mathbb{E}_{\mathcal{E}^{(n)}}\big[\|\Gamma_{W^n|\mathcal{E}^{(n)}} - \rho_{W}^{\otimes n}\|_{TV}\big] \underset{n \to \infty}{\longrightarrow} 0,$$
    \hfill\\
    where $\rho_W$ is the marginal of $\rho_{V,W} = \rho_V \cdot \rho_{W|V}.$
\end{lemma}
\hfill\\
We first use Lemma \ref{lemma:soft_covering} with $\rho = p,$ $\mathcal{E}^{(n)}=\mathcal{C}^{(n)},$ $k_n = \lfloor 2^{n(R+\varepsilon)}\rfloor \times \lfloor 2^{nR'}\rfloor \times \lfloor 2^{nR_c}\rfloor,$ $I=(M,M',J),$ $W^n=Y^n$ and $R$ replaced by $R+\varepsilon+R'+R_c.$ The corresponding output distribution is exactly $Q^{(1)}_{M,M',J, V^n, Y^n |\mathcal{C}^{(n)}= \cdot}$ thus by \eqref{eq:sum_rate_large_enough_for_Y} and Lemma \ref{lemma:soft_covering} together with the perception property $p_Y \equiv p_X$ from \eqref{eq:def_D_D} we get \eqref{eq:TV_Q_1_Y}.

Second, we use Lemma \ref{lemma:soft_covering} as follows. We fix a positive integer $j.$ For every $n$ such that $2^{nR_c}\geq j$ we set $\mathcal{E}^{(n)}$ to be the sub-codebook of $\mathcal{C}^{(n)}$ corresponding to $j$ and set $\rho = p,$ $k_n = \lfloor 2^{n(R+\varepsilon)}\rfloor \times \lfloor 2^{nR'}\rfloor.$ We further set $I=(M,M',j),$ $W=(X,Z)$ and replace $R$ in the lemma by $R+\varepsilon+R'.$ The corresponding output distribution is exactly $Q^{(1)}_{M,M', V^n, X^n, Z^n |\mathcal{C}^{(n)}= \cdot, J=j}$ thus by \eqref{eq:sum_rate_large_enough_for_X_and_Z} and Lemma \ref{lemma:soft_covering} we have
\begin{equation}\label{eq:TV_Q_1_X_Z}
    \forall j, \quad \mathbb{E}_{\mathcal{C}^{(n)}}\big[\|Q^{(1)}_{X^n, 
Z^n|\mathcal{C}^{(n)}, J=j} - p_{X, Z}^{\otimes n}\|_{TV}\big] \underset{n \to \infty}{\longrightarrow} 0.
\end{equation}

Moreover, since $Q^{(1)}_{\mathcal{C}^{(n)}, J} \equiv \mathbb{Q}_{\mathcal{C}^{(n)}}p^{\mathcal{U}}_{[2^{nR_c}]},$ then by Lemma \ref{lemma:get_expectation_out_of_TV} the total variation distance between
$Q^{(1)}_{\mathcal{C}^{(n)}, J, X^n, Z^n}$ and $\mathbb{Q}_{\mathcal{C}^{(n)}}p^{\mathcal{U}}_{[2^{nR_c}]}p_{X, Z}^{\otimes n}$ rewrites as
% \begin{IEEEeqnarray}{c}
% \mathbb{E}_{\mathcal{C}^{(n)}}\big[\|Q^{(1)}_{J, X^n, Z^n|\mathcal{C}^{(n)}} - p^{\mathcal{U}}_{[2^{nR_c}]}p_{X, Z}^{\otimes n}\|_{TV}\big]\nonumber
% \end{IEEEeqnarray}
\begin{IEEEeqnarray}{c}
    \sum_{j=1}^{\lfloor 2^{nR_c} \rfloor} \tfrac{\text{\normalsize 1}}{\lfloor 2^{nR_c} \rfloor} \mathbb{E}_{\mathcal{C}^{(n)}}\big[\|Q^{(1)}_{X^n, Z^n|\mathcal{C}^{(n)}, J=j} - p_{X, Z}^{\otimes n}\|_{TV}\big]. \nonumber
\end{IEEEeqnarray}
Finally, by construction of $\mathcal{C}^{(n)}$ the distribution of sub-codebooks $(V^n(\mathcal{C}^{(n)}, m,m',j))_{m,m'}$ is independent of $j.$ Hence all expectations in the above sum are identical. Using \eqref{eq:TV_Q_1_X_Z} we get \eqref{eq:TV_Q_1_J_X_Z}.

\subsubsection{Computations in the Gaussian case}\label{app:Gaussian}
% \subsubsection{Conditional mutual information computations in the converse proof}
\hfill\\
%\todo[inline]{In the converse, the definitions of Wyner are enough since I do not do any subtractions of mutual information terms and to deal with going from $t$ to $T$ I can do it for any discrete approximation.}
%\todo[inline]{Uniform integrability of Gaussian}
Since $\rho \geq \eta,$ we can choose
\begin{equation}\label{eq:def_b}
    b= \sqrt{(\rho^2 - \eta^2)/(1+\eta^2\rho^2-2\eta^2)}.
\end{equation}
We have $(X,Z) \sim p_{X,Z},$ the chain $Z-X-V$ and $I(Z;V) \leq h(Z) <\infty.$ By \eqref{eq:def_Z_X_V}, vector $(Z,X,V)$ is Gaussian and therefore
Then $Y$ is has normal distribution, which by \eqref{eq:rho_carre} is $\mathcal{N}(0,1) \equiv p_X$ and we have $X-(Z,V)-Y.$ 
\begin{lemma}
Let $(\Vec{x}_1, \Vec{x}_2)$ be a Gaussian vector with mean $(\Vec{\mu}_1, \Vec{\mu}_2)$ and covariance matrix \begin{equation*}
    \scalebox{0.9}{$\begin{pmatrix}
\Sigma_{11} & \Sigma_{12} \\
\Sigma_{21} & \Sigma_{12}
\end{pmatrix}$}
\end{equation*} Then, conditioned on $\Vec{x}_2\text{=}\Vec{a},$ variable $\Vec{x}_1$ is Gaussian with:
\begin{IEEEeqnarray}{c}
    \overline{\mu}_{|\Vec{a}} = \Vec{\mu}_1 + \Sigma_{12}\Sigma_{22}^{-1}(\Vec{a}-\Vec{\mu}_2)\label{eq:formula_conditiona_mean}\\
    \overline{\Sigma} = \Sigma_{11} - \Sigma_{12}\Sigma_{22}^{-1}\Sigma_{21},\label{eq:formula_conditiona_variance}
\end{IEEEeqnarray} with the covariance matrix $\overline{\Sigma}$ not depending on $\Vec{a}.$
\end{lemma}
For the centered Gaussian vector $(Z,X,V),$ we get
\begin{IEEEeqnarray}{c}
\text{Var}(X|Z) = 1 - \eta \cdot 1 \cdot \eta = 1-\eta^2 \text{ and}\label{eq:proved_Gaussian_Var_X_knowing_Z}\\
\mathbb{E}[X|Z,V]= 0 + \scalebox{0.9}{$\begin{pmatrix}
\eta & b
\end{pmatrix}$} \scalebox{0.9}{$\begin{pmatrix}
\tfrac{1}{1-\eta^2b^2} & \tfrac{-\eta b}{1-\eta^2b^2} \\
\tfrac{-\eta b}{1-\eta^2b^2} & \tfrac{1}{1-\eta^2b^2}
\end{pmatrix}$} \scalebox{0.9}{$\begin{pmatrix}
Z \\
V
\end{pmatrix}$}.\label{eq:gaussian_proof_conditional_mean}
%\\*
%&=& \dfrac{\eta-\eta b^2}{1-\eta^2 b^2}Z + \dfrac{b-\eta^2 b}{1-\eta^2 b^2}V.\label{eq:gaussian_proof_conditional_mean}
% \text{Var}[X|Z,V]= 1 - \scalebox{0.9}{$\begin{pmatrix}
% \eta & b
% \end{pmatrix}$} \scalebox{0.9}{$\begin{pmatrix}
% \tfrac{1}{1-\eta^2b^2} & \tfrac{-\eta b}{1-\eta^2b^2} \\
% \tfrac{-\eta b}{1-\eta^2b^2} & \tfrac{1}{1-\eta^2b^2}
% \end{pmatrix}$} \scalebox{0.9}{$\begin{pmatrix}
% \eta \\
% b
% \end{pmatrix}$} 
\end{IEEEeqnarray}
% \begin{IEEEeqnarray}{c}
%     \forall z, \text{Var}(X|Z=z) = 1-\eta^2 \text{ and}\label{eq:gaussian_Var_X_knowing_Z}\\*
%     \mathbb{E}[X|Z=z,V=v] = \dfrac{\eta-\eta b^2}{1-\eta^2 b^2}z + \dfrac{b-\eta^2 b}{1-\eta^2 b^2}v.\label{eq:conditional_expect_X_knowing_Z_V}
% \end{IEEEeqnarray}
%From \eqref{eq:def_Z_X_V}, \eqref{eq:def_b} and \eqref{eq:conditional_expect_X_knowing_Z_V}
%which prove \eqref{eq:gaussian_Var_X_knowing_Z} and \eqref{eq:conditional_expect_X_knowing_Z_V}. 
By \eqref{eq:def_Z_X_V}, $\mathbb{E}[Z^2]\text{=}\mathbb{E}[V^2]\text{=}1$ and $\mathbb{E}[ZV]\text{=}\eta b.$ Therefore, by \eqref{eq:gaussian_proof_conditional_mean} we have $\mathbb{E}[ \mathbb{E}[X|Z,V]^2]$
\begin{IEEEeqnarray}{rCl}
    &=& \dfrac{1}{(1\text{-}\eta^2 b^2)^2} \mathbb{E}\big[ [\eta(1\text{-}b^2)Z + b(1\text{-}\eta^2)V]^2 \big] \nonumber \\*
    &=& \dfrac{1}{(1\text{-}\eta^2 b^2)^2} \mathbb{E}\big[ \eta^2(1\text{-}b^2)^2 \text{+} b^2(1\text{-}\eta^2)^2 \text{+} 2\eta^2 b^2 (1\text{-}\eta^2)(1\text{-}b^2) \big]\IEEEeqnarraynumspace\label{eq:gaussian_developper_carre_rho_2}
\end{IEEEeqnarray}
Define $\lambda\text{=}1\text{-}\eta^2$ and $\tilde{\rho}\text{=}1-\rho^2.$ Then we have
\begin{IEEEeqnarray}{c}
    (1\text{+}\eta^2\rho^2\text{-}2\eta^2)b^2\text{=}\lambda\text{-}\tilde{\rho}, (1\text{+}\eta^2\rho^2\text{-}2\eta^2)(1\text{-}b^2)\text{=}\tilde{\rho}\lambda, \nonumber\\*
    (1\text{+}\eta^2\rho^2\text{-}2\eta^2)(1\text{-}\eta^2b^2)\text{=}\lambda^2, 1\text{+}\eta^2\rho^2\text{-}2\eta^2\text{=}\text{-}\tilde{\rho}\text{+}\lambda(1\text{+}\tilde{\rho}).\nonumber
\end{IEEEeqnarray}
Therefore, by multiplying numerator and denominator by $(1\text{+}\eta^2\rho^2\text{-}2\eta^2)^2$ in \eqref{eq:gaussian_developper_carre_rho_2} we get $\mathbb{E}[ \mathbb{E}[X|Z,V]^2]$
\begin{IEEEeqnarray}{rCl}
    &=& \dfrac{1}{\lambda^4}\Big[(1\text{-}\lambda)\tilde{\rho}^2\lambda^2\text{+}(\lambda\text{-}\tilde{\rho})\big[\text{-}\tilde{\rho}\text{+}\lambda(1\text{+}\tilde{\rho})\big]\lambda^2\text{+}2(1\text{-}\lambda)(\lambda\text{-}\tilde{\rho})\lambda\tilde{\rho}\lambda\Big] \nonumber \\*
    %&=& \scalebox{0.8}{$(1/\lambda^2)$}\Big[(1\text{-}\lambda)\tilde{\rho}^2\text{+}(\lambda\text{-}\tilde{\rho})\big[\text{-}\tilde{\rho}\text{+}\lambda(1\text{+}\tilde{\rho})\big]\text{+}2(1\text{-}\lambda)(\lambda\text{-}\tilde{\rho})\tilde{\rho}\Big]\nonumber\\*
    &=& \dfrac{1}{\lambda^2}\Big[(1\text{-}\lambda)\tilde{\rho}^2\text{+}\big[\tilde{\rho}^2\text{-}\lambda\tilde{\rho}(2\text{+}\tilde{\rho})\text{+}\lambda^2(1\text{+}\tilde{\rho})\big]\text{+}2\tilde{\rho}\big[\text{-}\tilde{\rho}\text{+}(1\text{+}\tilde{\rho})\lambda\text{-}\lambda^2\big]\Big]\nonumber\\*
    &=& \dfrac{1}{\lambda^2}\Big[1\cdot(\tilde{\rho}^2 \text{+} \tilde{\rho}^2 \text{-} 2\tilde{\rho}^2)+\lambda \cdot \big[\text{-}\tilde{\rho}^2\text{-}\tilde{\rho}(2\text{+}\tilde{\rho})\text{+}2\tilde{\rho}(1\text{+}\tilde{\rho})\big]\nonumber\\*
    &&\qquad \quad +\lambda^2\cdot\big[1\text{+}\tilde{\rho}\text{-}2\tilde{\rho}\big]\Big] \; = \tilde{\rho} = \rho^2.\nonumber
\end{IEEEeqnarray}
Finally, we compute $I(X;V|Z)$ and $\mathbb{E}[d(X,Y)].$ By translation invariance of differential entropy we have \begin{equation*}
    h(X|Z,V) = h\big(X\text{-}\mathbb{E}[X|Z,V]\big|Z,V\big).
\end{equation*}Since uncorrelated Gaussian vectors are independent, we get $h(X|Z,V) = h(X\text{-}\mathbb{E}[X|Z,V]).$ Since $\mathbb{E}[X^2]=1$ we get \begin{equation*}
    \text{Var}\big(X\text{-}\mathbb{E}[X|Z,V]\big) = 1 - \mathbb{E}[ \mathbb{E}[X|Z,V]^2].
\end{equation*}We then conclude the computation by \eqref{eq:proved_Gaussian_Var_X_knowing_Z} and \eqref{eq:rho_carre}. Also,
\begin{IEEEeqnarray}{rCl}
    \mathbb{E}[d(X,Y)] &=& \mathbb{E}[(X-\rho^{-1}\mathbb{E}[X|Z,V])^2] \nonumber \\*
    &=& 1 - 2\rho^{-1}\mathbb{E}\big[ \mathbb{E}[X|Z,V]^2 \big] + \rho^{-2}\mathbb{E}\big[ \mathbb{E}[X|Z,V]^2 \big] \nonumber \\*
    &=& 1-2\rho+1\nonumber\\*
    &=& \Delta.\label{eq:distortion_is_Delta}
\end{IEEEeqnarray}
The uniform integrability of $(d,p_X)$ is proved in \cite{2022AaronWagnerRDPTradeoffTheRoleOfCommonRandomness}. We recall the proof for completeness.\\
Let $X$ and $Y$ each have distribution $\mathcal{N}(m,\sigma^2)$ and $B$ be such that $\mathbb{P}(B)\leq \tau.$ Then by the Cauchy-Schwarz inequality:
\begin{IEEEeqnarray}{rCl}
    \mathbb{E}[(X-Y)^2\mathbf{1}_B] &\leq& \mathbb{E}[X^2]+\mathbb{E}[Y^2] + 2\mathbb{E}[(X\mathbf{1}_B)(Y\mathbf{1}_B)] \nonumber \\*
    &\leq& 2\sigma^2+ 2\sqrt{\mathbb{E}[X^2\mathbf{1}_B] \mathbb{E}[Y^2\mathbf{1}_B]}\nonumber \\*
    &\leq& 2\sigma^2+ 2\Big(\mathbb{E}[X^4]\mathbb{P}(B) \mathbb{E}[Y^4]\mathbb{P}(B)\Big)^{1/4}\nonumber\\*
    &\leq& 2\sigma^2+ 2\sqrt{\tau}\Big(\mathbb{E}[X^4] \mathbb{E}[Y^4]\Big)^{1/4}.\nonumber
\end{IEEEeqnarray} This concludes the proof since $\mathcal{N}(m,\sigma^2)$ has finite moments.

\todo[inline]{on the last page, the columns need to be balanced. Instructions for that purpose are given in the source file (they are commented out).}
