# Supplementary material for: The Rate-Distortion-Perception Trade-off with Side Information
Source: arXiv:2305.13116 source file (2023-05-22)
Supplement: Supplementary file 4 [file construction_P_2.tex]

\subsubsection{Modified code satisfying perfect realism}
\hfill\\
Consider the setting of Proposition \eqref{proposition:to_perfect_realism}. If $P^{(1)}_{Y^n} \equiv p_{X}^{\otimes n},$ we just set $P^{(2)} \equiv P^{(1)}.$ Assume this is not the case.
By Definition \ref{def:achievability}, the conditional distribution of $Y^n$ knowing all other variables reduces to $P^{(1)}_{Y^n|Z^n,M,J}.$ Let $\mu$ be $\sigma$-finite and dominating $P^{(1)}_{Y^n}$ and $p_{X}^{\otimes n},$ e.g. $P^{(1)}_{Y^n} + p_{X}^{\otimes n}.$ Let
\begin{IEEEeqnarray}{c}
    \mathcal{X}^n_{+} = \bigg\{ y^n \in \mathcal{X}^n \text{s.t.} \dfrac{dP^{(1)}_{Y^n}}{d\mu}(y^n) > \dfrac{dp_{X}^{\otimes n}}{d\mu}(y^n) \bigg\} \nonumber\\*
    \text{and } \theta_n: \mathcal{X}^n_{+} \to \mathbb{R}, y^n \mapsto \dfrac{dp_{X}^{\otimes n}/d\mu(y^n)}{dP^{(1)}_{Y^n}/d\mu(y^n)}.\nonumber
\end{IEEEeqnarray}
For any $z^n, m, j$ and any set $A \in \mathcal{X}^n$ we define
\begin{IEEEeqnarray}{rCl}
\IEEEeqnarraymulticol{3}{l}{
P^{(2)}(A |z^n, m, j) = P^{(1)}(A \backslash \mathcal{X}^n_{+} |z^n, m, j) \ +
}\nonumber\\*
& & \int_{A \cap \mathcal{X}^n_{+}} \theta_n(y^n) dP^{(1)}(y^n|z^n, m, j) + \phi_{z^n, m, j} \Gamma(A) \text{ where} \nonumber\\*
&&\Gamma(A) = \dfrac{\int_A (dp_{X}^{\otimes n}/d\mu(y^n) - dP^{(1)}_{Y^n}/d\mu(y^n))^{+} d\mu(y^n)}{\int (dp_{X}^{\otimes n}/d\mu(y^n) - dP^{(1)}_{Y^n}/d\mu(y^n))^{+} d\mu(y^n)}\nonumber\\*
&& \text{and } \phi_{z^n, m, j} = \int_{\mathcal{X}^n_{+}} 1 - \theta^n(y^n) dP^{(1)}(y^n|z^n, m, j). \label{eq:def_phi_bis}
\end{IEEEeqnarray}
It can be checked that this defines a probability measure for every $z^n, m, j.$ 
%The first two terms are non-negative measures because defined from non-negative density functions with respect to $P^{(1)}_{Y^n|Z^n, M, J}.$ The same applies to the third term defined with respect to $\mu,$ with the non-negativity of constant $\phi_{z^n, m, j}$ coming from the fact that by definition we have $\theta^n < 1$ on $\mathcal{X}^n_{+}.$ Finally we have $\Gamma(\mathcal{X}^n)=1,$ giving $P^{(2)}(\mathcal{X}^n|z^n, m, j) = 1.$ 
We define the joint distribution for the new code as
\begin{equation}\label{eq:def_P_2_bis}
    P^{(2)}_{\scalebox{0.7}{$X^n, Z^n, M, J, Y^n$}} = P^{(1)}_{\scalebox{0.7}{$X^n, Z^n, M, J$}}P^{(2)}_{\scalebox{0.7}{$Y^n| Z^n, M, J$}}.
\end{equation}
% \begin{IEEEeqnarray}{rCl}
% \IEEEeqnarraymulticol{3}{l}{
% P^{(2)}(\mathcal{X}^n|z^n, m, j) = P^{(1)}(\mathcal{X}^n \backslash \mathcal{X}^n_{+} |z^n, m, j) \ +
% }\nonumber\\*
% & & \int_{ \mathcal{X}^n_{+}} \theta_n(y^n) dP^{(1)}(y^n|z^n, m, j) + \int_{\mathcal{X}^n_{+}} 1 - \theta^n(y^n) dP^{(1)}(y^n|z^n, m, j) \nonumber\\*
% &&\nonumber\\*
% && . \nonumber\end{IEEEeqnarray}
Then similarly to $P^{(1)},$ $P^{(2)}$ is the distribution induced by a $(n,R,R_c)$ D(resp. E-D)-code. Moreover the latter has the same encoder as $P^{(1)}.$ Based on this and since the definition of $P^{(2)}(\cdot | z^n, m, j)$ is affine in $P^{(1)}(\cdot | z^n, m, j),$ one can show that $P^{(2)}$ satisfies perfect realism by taking the expectation according to $P^{(1)}_{Z^n, M, J}$ and using Fubini's theorem for non-negative variables.
% \begin{IEEEeqnarray}{rCl}
% P^{(2)}_{Y^n}(A) &=& P^{(1)}_{Y^n}(A \backslash \mathcal{X}^n_{+}) \ + \int_{A \cap \mathcal{X}^n_{+}} \theta_n(y^n) dP^{(1)}_{Y^n}(y^n) \nonumber\\*
% & + &  \Gamma(A) \int_{\mathcal{X}^n_{+}} 1 - \theta^n(y^n) dP^{(1)}_{Y^n}(y^n) \nonumber\\*
% &=& P^{(1)}_{Y^n}(A \backslash \mathcal{X}^n_{+}) \ + p_{X}^{\otimes n}(A \cap \mathcal{X}^n_{+})  \nonumber\\*
% & + &  \Gamma(A) \int_{\mathcal{X}^n_{+}} \tfrac{dP^{(1)}_{Y^n}}{d\mu}(y^n) - \tfrac{dp_{X}^{\otimes n}}{d\mu}(y^n) d\mu(y^n) \nonumber.
% \end{IEEEeqnarray} By definition of $\mathcal{X}^n_{+},$ the last term reduces to the numerator of $\Gamma(A),$ which reduces to 
% \begin{IEEEeqnarray}{rCl}
% \IEEEeqnarraymulticol{3}{l}{
% \int_{A \backslash \mathcal{X}^n_{+}} \tfrac{dp_{X}^{\otimes n}}{d\mu}(y^n) - \tfrac{dP^{(1)}_{Y^n}}{d\mu}(y^n) d\mu(y^n)
% }\nonumber\\*
% & = & p_{X}^{\otimes n}(A \backslash \mathcal{X}^n_{+}) - P^{(1)}_{Y^n}(A \backslash \mathcal{X}^n_{+}). \nonumber
% \end{IEEEeqnarray}
The last step consists in obtaining the distortion bound by coupling $P^{(2)}$ with $Q.$\\
