# Supplementary material for: The Rate-Distortion-Perception Trade-off with Side Information
Source: arXiv:2305.13116 source file (2023-05-22)
Supplement: Supplementary file 5 [file coupling.tex]

\subsubsection{Coupling with $Q$}
\hfill\\
We first compare $P^{(2)}$ to $P^{(1)}.$ For every $z^n, m, j$ and every set $A \in \mathcal{X}^n$ we have:
\begin{IEEEeqnarray}{rCl}
\IEEEeqnarraymulticol{3}{l}{
P^{(1)}(A |z^n, m, j) - P^{(2)}(A |z^n, m, j)
}\nonumber\\*
& = & \int_{A \cap \mathcal{X}^n_{+}} 1 - \theta_n(y^n) dP^{(1)}(y^n|z^n, m, j) - \phi_{z^n, m, j} \Gamma(A). \nonumber
\end{IEEEeqnarray} Both terms being smaller than or equal to $\phi_{z^n, m, j},$ we have
\begin{IEEEeqnarray}{c}
    \big\|P^{(2)}_{Y^n|Z^n\text{=}z^n, M\text{=}m, J\text{=}j} - P^{(1)}_{Y^n|Z^n\text{=}z^n, M\text{=}m, J\text{=}j}\big\|_{TV} \leq \phi_{z^n, m, j}.\nonumber
\end{IEEEeqnarray}
When integrating this over all variables except $Y^n,$ we get by definition \eqref{eq:def_P_2_bis} of $P^{(2)}$ and Lemma \ref{lemma:get_expectation_out_of_TV} on the one hand and by definition \eqref{eq:def_phi_bis} of $\phi$ and Fubini's theorem on the other hand:
\begin{IEEEeqnarray}{rCl}
\IEEEeqnarraymulticol{3}{l}{
\big\|P^{(2)}_{\scalebox{0.6}{$X^n, Z^n, M, J, Y^n$}} - P^{(1)}_{\scalebox{0.6}{$X^n, Z^n, M, J, Y^n$}}\big\|_{TV}
}\nonumber\\*
%& \leq & \int \phi_{z^n, m, j} dP^{(1)}_{\scalebox{0.6}{$X^n, Z^n, M, J$}} \nonumber\\*
&\leq& \int_{\mathcal{X}^n_{+}} 1 - \theta^n(y^n) dP^{(1)}_{Y^n}(y^n) = \big\|P^{(1)}_{Y^n} - p_{X}^{\otimes n} \big\|_{TV}.\nonumber
\end{IEEEeqnarray}
Therefore by Lemma \ref{lemma:TV_joint_to_TV_marginal} applied to assumption \eqref{eq:total_variation_Q_P_assumption_theorem_to_perfect_realism} with $W=Y^n$ and by the triangle inequality and assumption \eqref{eq:perception_assumption_theorem_to_perfect_realism} we get
\begin{IEEEeqnarray}{c}
    \big\|P^{(2)}_{\scalebox{0.6}{$X^n, Z^n, M, J, Y^n$}} - P^{(1)}_{\scalebox{0.6}{$X^n, Z^n, M, J, Y^n$}}\big\|_{TV} \leq \varepsilon_2 + \varepsilon_3.\nonumber
\end{IEEEeqnarray}
Therefore by Lemma \ref{lemma:TV_joint_to_TV_marginal} with $W=(X^n, Y^n)$ and $W=Y^n$ and the triangle inequality with assumption \eqref{eq:total_variation_Q_P_assumption_theorem_to_perfect_realism} we get
\begin{IEEEeqnarray}{c}
    \big\|P^{(2)}_{X^n,Y^n} - Q_{X^n,Y^n}\big\|_{TV} \leq \varepsilon_2 + 2\varepsilon_3. \IEEEeqnarraynumspace \label{eq:TV_on_X_and_Y_P_2_Q_anonymous}
\end{IEEEeqnarray}
We then use the following standard coupling lemma (see e.g. \cite[Chapter~I, Theorem~5.2]{1992Coupling_Book}):
% \begin{lemma}\label{lemma:coupling_existence_bis}
% For any two probability measures $\Pi, \Pi'$ on a measurable space there exists a probability measure $\rho$ and a random tuple $(W,W')$ with distribution $\rho$ with marginals $\rho_W \equiv \Pi$ and $\rho_{W'} \equiv \Pi'$ and such that $\rho(W \neq W') = \|\Pi - \Pi'\|_{TV}.$
% \end{lemma}
%Thus 
by \eqref{eq:TV_on_X_and_Y_P_2_Q_anonymous} there exists a quadruple $(X^n, Y^n, \Tilde{X}^n, \Tilde{Y}^n)$ with distribution denoted by $\rho$ having marginals $P^{(2)}_{X^n,Y^n}$ and $Q_{X^n,Y^n}$ and such that $\rho((X^n, Y^n)\neq (\Tilde{X}^n, \Tilde{Y}^n)) \leq \varepsilon_2 + 2\varepsilon_3.$ We then have
\begin{IEEEeqnarray}{rCl}
\IEEEeqnarraymulticol{3}{l}{
\mathbb{E}_{P^{(2)}}[d(X^n, Y^n)] = \mathbb{E}_{\rho}[d(X^n, Y^n)]
}\nonumber\\*
&=& \mathbb{E}_{\rho}\Big[d(\Tilde{X}^n, \Tilde{Y}^n)\substack{\scalebox{1.0}{$\mathbf{1} \qquad \qquad \qquad \quad$}  \\ (X^n, Y^n) = (\Tilde{X}^n, \Tilde{Y}^n)}\Big] \nonumber \\*
&+& \mathbb{E}_{\rho}\Big[d(X^n, Y^n)\substack{\scalebox{1.0}{$\mathbf{1} \qquad \qquad \qquad \quad$}  \\ (X^n, Y^n) \neq (\Tilde{X}^n, \Tilde{Y}^n)}\Big] \nonumber\\*
&\leq& \mathbb{E}_{Q}[d(X^n, Y^n)] + \tfrac{1}{n}\sum_{i=1}^n \mathbb{E}_{\rho}\Big[d(X_i, Y_i)\substack{\scalebox{1.0}{$\mathbf{1} \qquad \qquad \qquad \quad$}  \\ (X^n, Y^n) \neq (\Tilde{X}^n, \Tilde{Y}^n)}\Big]\nonumber\\*
&\leq& \mathbb{E}_{Q}[d(X^n, Y^n)] + \tfrac{1}{n}\sum_{i=1}^n \sup_{X,Y,B}\mathbb{E}\Big[d(X, Y) \ \scalebox{1.0}{$\mathbf{1}_B $}\Big], \nonumber
\end{IEEEeqnarray} the supremum is over all variables $X$ and $Y$ having law $p_X$ and all events $B$ with $\rho(B) \leq \varepsilon_2 + 2\varepsilon_3,$ and the last inequality holds because $P^{(2)}$ satisfies perfect realism $P^{(2)}_{Y^n} = p_X^{\otimes n}$ and by \eqref{eq:def_P_2_bis} we have $P^{(2)}_{X^n} = p_X^{\otimes n}.$ We conclude by assumption \eqref{eq:distortion_assumption_theorem_to_perfect_realism}.
