# Supplementary material for: The Rate-Distortion-Perception Trade-off with Side Information
Source: arXiv:2305.13116 source file (2023-05-22)
Supplement: Supplementary file 6 [file main_file_simple_justifications_and_computations.tex]

\subsection{Further justifications}
\subsubsection{Equivalence between achievability with near-perfect and perfect realism}\label{app:equivalence_perfect_realism}
\hfill\\
In order to prove Theorem \ref{theorem:equivalence_perfect_realism}, we state the following result, which corresponds to Remark \ref{remark:existence_of_prop_to_perfect_realism} and which we also use in Section \ref{sec:achievability}.
\begin{proposition}\label{proposition:to_perfect_realism}
Let $n$ be a positive integer and $\varepsilon_1, \varepsilon_2, \varepsilon_3$ be positive reals. Let $\mathcal{X}$ and $\mathcal{Z}$ be two Polish alphabets and $p_{X,Z}$ be a joint distribution on $\mathcal{X} \times \mathcal{Z}.$ 
%dominated by a product of $\sigma$-finite measures $\mu$ and $\gamma.$ 
Let $d$ be a distortion measure such that $(d,p_X)$ is uniformly integrable. Let $Q_{X^n, Y^n}$ be a distribution on $\mathcal{X}^n \times \mathcal{X}^n$ satisfying
\begin{IEEEeqnarray}{rCl}
\IEEEeqnarraymulticol{3}{l}{
\mathbb{E}_Q[d(X^n, Y^n)] \leq \Delta + \varepsilon_1 
} \label{eq:distortion_assumption_theorem_to_perfect_realism}\\*
&\text{ and } \| Q_{Y^n} - p_X^{\otimes n} \|_{TV} \leq \varepsilon_2.& \label{eq:perception_assumption_theorem_to_perfect_realism}
\end{IEEEeqnarray} Let $P^{(1)}$ be a distribution induced (Definition \ref{def:achievability}) by a $(n,R,R_c)$ D-code (resp. E-D-code) for some reals $R,R_c\geq 0.$ Assume that \begin{equation}
    \| P^{(1)}_{X^n, Y^n} - Q_{X^n, Y^n} \|_{TV} \leq \varepsilon_3.\label{eq:total_variation_Q_P_assumption_theorem_to_perfect_realism}
\end{equation} Then there is a $(n,R,R_c)$ D-code (resp. E-D-code) with the same encoder as $P^{(1)}$ and inducing a distribution $P^{(2)}$ with
\begin{IEEEeqnarray}{rCl}
\IEEEeqnarraymulticol{3}{l}{
\mathbb{E}_{P^{(2)}}[d(X^n, Y^n)] \leq \Delta + \varepsilon_1 + \sup_{X,Y,B}\mathbb{E}[d(X, Y) \ \scalebox{1.0}{$\mathbf{1}_B $}]
} \label{eq:distortion_result_theorem_to_perfect_realism}\\*
&\text{ and } P^{(2)}_{Y^n} \equiv p_X^{\otimes n},& \label{eq:perception_result_theorem_to_perfect_realism}
\end{IEEEeqnarray} where the supremum is over all variables $X$ and $Y$ having law $p_X$ and all events $B$ with probability at most $\varepsilon_2 + 2\varepsilon_3.$
\end{proposition}
\vspace{5pt}
%We start by showing how 
Proposition \ref{proposition:to_perfect_realism} implies Theorem \ref{theorem:equivalence_perfect_realism} by taking $Q\equiv P^{(1)}$ at fixed blocklength.
% \begin{IEEEproof}
% We know that the D(resp. E-D)-achievability with perfect realism implies that with near-perfect realism. Consider a triplet $(R,R_c,\Delta)$ D(resp. E-D)-achievable with near-perfect realism and a corresponding sequence of $(n, R, R_c)$ codes $(F^{(n)},G^{(n)})_n.$ 
% %and two vanishing sequences $(\varepsilon_{1,n})_n, (\varepsilon_{2,n})_n$ of positive reals such that for every $n,$
% %\begin{IEEEeqnarray}{rCl}
% %\IEEEeqnarraymulticol{3}{l}{
% %\mathbb{E}_{P^{(n)}}[d(X^n, Y^n)] \leq \Delta + \varepsilon_{1,n} 
% %} \\*
% %\text{ and } \| P^{(n)}_{Y^n} - p_X^{\otimes n} \|_{TV} \leq %\varepsilon_{2,n}.&& 
% %\end{IEEEeqnarray}
% Then the achievability with perfect realism is obtained by using Proposition \ref{proposition:to_perfect_realism} with the $Q\equiv P^{(1)}$ and equal to the distribution induced by the $n$-th code, and by the uniform integrability assumption.
% %$\varepsilon_1=\varepsilon_{1,n}, \varepsilon_2=\varepsilon_{2,n}, \varepsilon_3=0,$ there exists a sequence of codes and their corresponding distributions $(\Tilde{P}^{(n)})_n$ such that for all $n$
% % \begin{IEEEeqnarray}{rCl}
% % \IEEEeqnarraymulticol{3}{l}{
% % \mathbb{E}_{\Tilde{P}^{(n)}}[d(X^n, Y^n)] \leq \Delta + \varepsilon_{1,n} + \varepsilon_{2,n}
% % } \label{eq:distortion_result_theorem_to_perfect_realism}\\*
% % &\text{ and } \Tilde{P}^{(n)}_{Y^n} \equiv p_X^{\otimes n}.& \label{eq:perception_result_theorem_to_perfect_realism}
% % \end{IEEEeqnarray}
% \end{IEEEproof}
%We now prove Proposition \ref{proposition:to_perfect_realism} and divide the proof in two parts.\\
We prove Proposition \ref{proposition:to_perfect_realism} in the next two subsections.
\subsubsection{Modified code satisfying perfect realism}
\hfill\\
Consider the setting of Proposition \eqref{proposition:to_perfect_realism}. If $P^{(1)}_{Y^n} \equiv p_{X}^{\otimes n},$ we just set $P^{(2)} \equiv P^{(1)}.$ Assume this is not the case.
By Definition \ref{def:achievability}, the conditional distribution of $Y^n$ knowing all other variables reduces to $P^{(1)}_{Y^n|Z^n,M,J}.$ Let $\mu$ be $\sigma$-finite and dominating $P^{(1)}_{Y^n}$ and $p_{X}^{\otimes n},$ e.g. $P^{(1)}_{Y^n} + p_{X}^{\otimes n}.$ Let
\begin{IEEEeqnarray}{c}
    \mathcal{X}^n_{+} = \bigg\{ y^n \in \mathcal{X}^n \text{s.t.} \dfrac{dP^{(1)}_{Y^n}}{d\mu}(y^n) > \dfrac{dp_{X}^{\otimes n}}{d\mu}(y^n) \bigg\} \nonumber\\*
    \text{and } \theta_n: \mathcal{X}^n_{+} \to \mathbb{R}, y^n \mapsto \dfrac{dp_{X}^{\otimes n}/d\mu(y^n)}{dP^{(1)}_{Y^n}/d\mu(y^n)}.\nonumber
\end{IEEEeqnarray}
For any $z^n, m, j$ and any set $A \in \mathcal{X}^n$ we define
\begin{IEEEeqnarray}{rCl}
\IEEEeqnarraymulticol{3}{l}{
P^{(2)}(A |z^n, m, j) = P^{(1)}(A \backslash \mathcal{X}^n_{+} |z^n, m, j) \ +
}\nonumber\\*
& & \int_{A \cap \mathcal{X}^n_{+}} \theta_n(y^n) dP^{(1)}(y^n|z^n, m, j) + \phi_{z^n, m, j} \Gamma(A) \text{ where} \nonumber\\*
&&\Gamma(A) = \dfrac{\int_A (dp_{X}^{\otimes n}/d\mu(y^n) - dP^{(1)}_{Y^n}/d\mu(y^n))^{+} d\mu(y^n)}{\int (dp_{X}^{\otimes n}/d\mu(y^n) - dP^{(1)}_{Y^n}/d\mu(y^n))^{+} d\mu(y^n)}\nonumber\\*
&& \text{and } \phi_{z^n, m, j} = \int_{\mathcal{X}^n_{+}} 1 - \theta^n(y^n) dP^{(1)}(y^n|z^n, m, j). \label{eq:def_phi_bis}
\end{IEEEeqnarray}
It can be checked that this defines a probability measure for every $z^n, m, j.$ 
%The first two terms are non-negative measures because defined from non-negative density functions with respect to $P^{(1)}_{Y^n|Z^n, M, J}.$ The same applies to the third term defined with respect to $\mu,$ with the non-negativity of constant $\phi_{z^n, m, j}$ coming from the fact that by definition we have $\theta^n < 1$ on $\mathcal{X}^n_{+}.$ Finally we have $\Gamma(\mathcal{X}^n)=1,$ giving $P^{(2)}(\mathcal{X}^n|z^n, m, j) = 1.$ 
We define the joint distribution for the new code as
\begin{equation}\label{eq:def_P_2_bis}
    P^{(2)}_{\scalebox{0.7}{$X^n, Z^n, M, J, Y^n$}} = P^{(1)}_{\scalebox{0.7}{$X^n, Z^n, M, J$}}P^{(2)}_{\scalebox{0.7}{$Y^n| Z^n, M, J$}}.
\end{equation}
% \begin{IEEEeqnarray}{rCl}
% \IEEEeqnarraymulticol{3}{l}{
% P^{(2)}(\mathcal{X}^n|z^n, m, j) = P^{(1)}(\mathcal{X}^n \backslash \mathcal{X}^n_{+} |z^n, m, j) \ +
% }\nonumber\\*
% & & \int_{ \mathcal{X}^n_{+}} \theta_n(y^n) dP^{(1)}(y^n|z^n, m, j) + \int_{\mathcal{X}^n_{+}} 1 - \theta^n(y^n) dP^{(1)}(y^n|z^n, m, j) \nonumber\\*
% &&\nonumber\\*
% && . \nonumber\end{IEEEeqnarray}
Then similarly to $P^{(1)},$ $P^{(2)}$ is the distribution induced by a $(n,R,R_c)$ D(resp. E-D)-code. Moreover the latter has the same encoder as $P^{(1)}.$ Based on this and since the definition of $P^{(2)}(\cdot | z^n, m, j)$ is affine in $P^{(1)}(\cdot | z^n, m, j),$ one can show that $P^{(2)}$ satisfies perfect realism by taking the expectation according to $P^{(1)}_{Z^n, M, J}$ and using Fubini's theorem for non-negative variables.
% \begin{IEEEeqnarray}{rCl}
% P^{(2)}_{Y^n}(A) &=& P^{(1)}_{Y^n}(A \backslash \mathcal{X}^n_{+}) \ + \int_{A \cap \mathcal{X}^n_{+}} \theta_n(y^n) dP^{(1)}_{Y^n}(y^n) \nonumber\\*
% & + &  \Gamma(A) \int_{\mathcal{X}^n_{+}} 1 - \theta^n(y^n) dP^{(1)}_{Y^n}(y^n) \nonumber\\*
% &=& P^{(1)}_{Y^n}(A \backslash \mathcal{X}^n_{+}) \ + p_{X}^{\otimes n}(A \cap \mathcal{X}^n_{+})  \nonumber\\*
% & + &  \Gamma(A) \int_{\mathcal{X}^n_{+}} \tfrac{dP^{(1)}_{Y^n}}{d\mu}(y^n) - \tfrac{dp_{X}^{\otimes n}}{d\mu}(y^n) d\mu(y^n) \nonumber.
% \end{IEEEeqnarray} By definition of $\mathcal{X}^n_{+},$ the last term reduces to the numerator of $\Gamma(A),$ which reduces to 
% \begin{IEEEeqnarray}{rCl}
% \IEEEeqnarraymulticol{3}{l}{
% \int_{A \backslash \mathcal{X}^n_{+}} \tfrac{dp_{X}^{\otimes n}}{d\mu}(y^n) - \tfrac{dP^{(1)}_{Y^n}}{d\mu}(y^n) d\mu(y^n)
% }\nonumber\\*
% & = & p_{X}^{\otimes n}(A \backslash \mathcal{X}^n_{+}) - P^{(1)}_{Y^n}(A \backslash \mathcal{X}^n_{+}). \nonumber
% \end{IEEEeqnarray}
The last step consists in obtaining the distortion bound by coupling $P^{(2)}$ with $Q.$\\
\subsubsection{Coupling with $Q$}
\hfill\\
We first compare $P^{(2)}$ to $P^{(1)}.$ For every $z^n, m, j$ and every set $A \in \mathcal{X}^n$ we have:
\begin{IEEEeqnarray}{rCl}
\IEEEeqnarraymulticol{3}{l}{
P^{(1)}(A |z^n, m, j) - P^{(2)}(A |z^n, m, j)
}\nonumber\\*
& = & \int_{A \cap \mathcal{X}^n_{+}} 1 - \theta_n(y^n) dP^{(1)}(y^n|z^n, m, j) - \phi_{z^n, m, j} \Gamma(A). \nonumber
\end{IEEEeqnarray} Both terms being smaller than or equal to $\phi_{z^n, m, j},$ we have
\begin{IEEEeqnarray}{c}
    \big\|P^{(2)}_{Y^n|Z^n\text{=}z^n, M\text{=}m, J\text{=}j} - P^{(1)}_{Y^n|Z^n\text{=}z^n, M\text{=}m, J\text{=}j}\big\|_{TV} \leq \phi_{z^n, m, j}.\nonumber
\end{IEEEeqnarray}
When integrating this over all variables except $Y^n,$ we get by definition \eqref{eq:def_P_2_bis} of $P^{(2)}$ and Lemma \ref{lemma:get_expectation_out_of_TV} on the one hand and by definition \eqref{eq:def_phi_bis} of $\phi$ and Fubini's theorem on the other hand:
\begin{IEEEeqnarray}{rCl}
\IEEEeqnarraymulticol{3}{l}{
\big\|P^{(2)}_{\scalebox{0.6}{$X^n, Z^n, M, J, Y^n$}} - P^{(1)}_{\scalebox{0.6}{$X^n, Z^n, M, J, Y^n$}}\big\|_{TV}
}\nonumber\\*
%& \leq & \int \phi_{z^n, m, j} dP^{(1)}_{\scalebox{0.6}{$X^n, Z^n, M, J$}} \nonumber\\*
&\leq& \int_{\mathcal{X}^n_{+}} 1 - \theta^n(y^n) dP^{(1)}_{Y^n}(y^n) = \big\|P^{(1)}_{Y^n} - p_{X}^{\otimes n} \big\|_{TV}.\nonumber
\end{IEEEeqnarray}
Therefore by Lemma \ref{lemma:TV_joint_to_TV_marginal} applied to assumption \eqref{eq:total_variation_Q_P_assumption_theorem_to_perfect_realism} with $W=Y^n$ and by the triangle inequality and assumption \eqref{eq:perception_assumption_theorem_to_perfect_realism} we get
\begin{IEEEeqnarray}{c}
    \big\|P^{(2)}_{\scalebox{0.6}{$X^n, Z^n, M, J, Y^n$}} - P^{(1)}_{\scalebox{0.6}{$X^n, Z^n, M, J, Y^n$}}\big\|_{TV} \leq \varepsilon_2 + \varepsilon_3.\nonumber
\end{IEEEeqnarray}
Therefore by Lemma \ref{lemma:TV_joint_to_TV_marginal} with $W=(X^n, Y^n)$ and $W=Y^n$ and the triangle inequality with assumption \eqref{eq:total_variation_Q_P_assumption_theorem_to_perfect_realism} we get
\begin{IEEEeqnarray}{c}
    \big\|P^{(2)}_{X^n,Y^n} - Q_{X^n,Y^n}\big\|_{TV} \leq \varepsilon_2 + 2\varepsilon_3. \IEEEeqnarraynumspace \label{eq:TV_on_X_and_Y_P_2_Q_anonymous}
\end{IEEEeqnarray}
We then use the following standard coupling lemma (see e.g. \cite[Chapter~I, Theorem~5.2]{1992Coupling_Book}):
% \begin{lemma}\label{lemma:coupling_existence_bis}
% For any two probability measures $\Pi, \Pi'$ on a measurable space there exists a probability measure $\rho$ and a random tuple $(W,W')$ with distribution $\rho$ with marginals $\rho_W \equiv \Pi$ and $\rho_{W'} \equiv \Pi'$ and such that $\rho(W \neq W') = \|\Pi - \Pi'\|_{TV}.$
% \end{lemma}
%Thus 
by \eqref{eq:TV_on_X_and_Y_P_2_Q_anonymous} there exists a quadruple $(X^n, Y^n, \Tilde{X}^n, \Tilde{Y}^n)$ with distribution denoted by $\rho$ having marginals $P^{(2)}_{X^n,Y^n}$ and $Q_{X^n,Y^n}$ and such that $\rho((X^n, Y^n)\neq (\Tilde{X}^n, \Tilde{Y}^n)) \leq \varepsilon_2 + 2\varepsilon_3.$ We then have
\begin{IEEEeqnarray}{rCl}
\IEEEeqnarraymulticol{3}{l}{
\mathbb{E}_{P^{(2)}}[d(X^n, Y^n)] = \mathbb{E}_{\rho}[d(X^n, Y^n)]
}\nonumber\\*
&=& \mathbb{E}_{\rho}\Big[d(\Tilde{X}^n, \Tilde{Y}^n)\substack{\scalebox{1.0}{$\mathbf{1} \qquad \qquad \qquad \quad$}  \\ (X^n, Y^n) = (\Tilde{X}^n, \Tilde{Y}^n)}\Big] \nonumber \\*
&+& \mathbb{E}_{\rho}\Big[d(X^n, Y^n)\substack{\scalebox{1.0}{$\mathbf{1} \qquad \qquad \qquad \quad$}  \\ (X^n, Y^n) \neq (\Tilde{X}^n, \Tilde{Y}^n)}\Big] \nonumber\\*
&\leq& \mathbb{E}_{Q}[d(X^n, Y^n)] + \tfrac{1}{n}\sum_{i=1}^n \mathbb{E}_{\rho}\Big[d(X_i, Y_i)\substack{\scalebox{1.0}{$\mathbf{1} \qquad \qquad \qquad \quad$}  \\ (X^n, Y^n) \neq (\Tilde{X}^n, \Tilde{Y}^n)}\Big]\nonumber\\*
&\leq& \mathbb{E}_{Q}[d(X^n, Y^n)] + \tfrac{1}{n}\sum_{i=1}^n \sup_{X,Y,B}\mathbb{E}\Big[d(X, Y) \ \scalebox{1.0}{$\mathbf{1}_B $}\Big], \nonumber
\end{IEEEeqnarray} the supremum is over all variables $X$ and $Y$ having law $p_X$ and all events $B$ with $\rho(B) \leq \varepsilon_2 + 2\varepsilon_3,$ and the last inequality holds because $P^{(2)}$ satisfies perfect realism $P^{(2)}_{Y^n} = p_X^{\otimes n}$ and by \eqref{eq:def_P_2_bis} we have $P^{(2)}_{X^n} = p_X^{\otimes n}.$ We conclude by assumption \eqref{eq:distortion_assumption_theorem_to_perfect_realism}.

\subsubsection{Proof of Corollary \ref{corollary:E_D_rates_region}}\label{app:proof_corollary}
\hfill\\
Consider the setting of the corollary. Let $(X,Z)$ be a couple with distribution $p_{X,Z}$ and let $\Tilde{\mathcal{X}} = \mathcal{X} \times \mathcal{Z},$ $\Tilde{\mathcal{Z}} = \mathcal{Z},$ $\Tilde{X} = (X,Z),$ $\Tilde{Z} = Z$ and $\Tilde{p}_{\Tilde{X}, \Tilde{Z}}.$ Define \begin{equation*}
\Tilde{d}: \Tilde{\mathcal{X}} \times \Tilde{\mathcal{X}} \to [0,\infty), \quad (x,z,x',z') \mapsto d(x,x')   
\end{equation*} These new objects statisfy the conditions of Theorem \ref{theorem:D_rates_region}: $(\Tilde{d}, \Tilde{p}_{\Tilde{X}})$ is uniformly integrable because $(d, p_X)$ is. Denote by $\Tilde{\mathcal{S}}_{D,\infty}$ the corresponding region. By Theorem \ref{theorem:equivalence_perfect_realism}, D(resp. E-D)-achievability with near perfect realism is equivalent to D(resp. E-D)-achievability with perfect realism. The latter notion will be used hereafter. Given a D-code for $(\Tilde{d}, \Tilde{p}_{\Tilde{X}, \Tilde{Z}}),$ applying the projection $\pi: (x,z) \mapsto (x',z')$ after the decoder gives a E-D-code for $(d,p_{X,Z}).$ Hence, by Lemma \ref{lemma:TV_joint_to_TV_marginal}, a D-achievable couple $(R,\Delta)$ for $(\Tilde{d}, \Tilde{p}_{\Tilde{X}, \Tilde{Z}})$ is also E-D-achievable for $(d,p_{X,Z}).$ Moreover, given a E-D-achievable couple $(R,\Delta)$ for $(d,p_{X,Z})$ and a corresponding sequence of E-D-codes $(F_n, G_n),$ modifying the decoder to $G^{(n)}_{Y^n|Z^n, J, M} \cdot \prod_{k=1}^n p_{Z|X=Y_k}$ gives a sequences of codes attesting the D-achievability of $(R,\Delta)$ for $(\Tilde{d}, \Tilde{p}_{\Tilde{X}, \Tilde{Z}}).$ Hence Corollary \ref{corollary:E_D_rates_region} holds with $\mathcal{S}_{E\text{-}D,\infty} = \Tilde{\mathcal{S}}_{D,\infty}:$
\begin{align}\label{eq:def_S_E_D_infty_bis}
      & 
    \left\{ \begin{array}{rcl}
        (R, \Delta) \in \mathbb{R}_{\geq 0}^2 &:& \exists \ \Tilde{p}_{X,Z,\Tilde{V},\hat{X}, \hat{Z}} \in \Tilde{D}_D \text{ s.t. } \\
        R &\geq& I_{\Tilde{p}}(\Tilde{V};X|Z) \\
        \Delta &\geq& \mathbb{E}_{\Tilde{p}}[d(X, \hat{X})]
    \end{array}\right\}, 
\end{align}
with $\Tilde{D}_D$ being
\begin{align}\label{eq:def_D_E_D_bis}
       & 
    \left\{ \begin{array}{rcl}
        &\Tilde{p}_{X,Z,\Tilde{V},\hat{X}, \hat{Z}} : \scalebox{0.9}{$(X,Z) \sim$ } p_{X,Z}& \\
        &\Tilde{p}_{\hat{X}, \hat{Z}} \equiv p_{X, Z}&\\
        &X - (Z, \Tilde{V}) - (\hat{X}, \hat{Z})& \\
        &I_{\Tilde{p}}(Z;\Tilde{V}) < \infty&
        %\exists \nu \ \sigma\text{-finite s.t. }& p \ll & \mu \times \gamma \times \nu \times \mu
    \end{array}\right\},
\end{align} where $\Tilde{Y}$ has been replaced by $(\hat{X}, \hat{Z}),$ $I(\Tilde{X}; \Tilde{V}|\Tilde{Z}) = (X,Z;\Tilde{V}|Z) = I(X;\Tilde{V}|Z)$ and the Markov chain $\Tilde{Z}-\Tilde{X}-\Tilde{V}$ is trivial and has been omitted. The region $\Tilde{\mathcal{S}}_{D,\infty}$ is unchanged when replacing $\Tilde{\mathcal{D}}_D$ in \eqref{eq:def_S_E_D_infty_bis} by its successive images through the following maps, which preserve $\mathbb{E}_{\Tilde{p}}[d(X, \hat{X})]$ and 
%diminishes 
$I_{\Tilde{p}}(\Tilde{V};X|Z):$ 
%to $I_{\Tilde{p}}(\hat{X};X|Z)$ (data processing inequality):
\begin{equation*}
    \Tilde{p}_{X,Z,\Tilde{V},\hat{X}, \hat{Z}} \mapsto \Tilde{p}_{X,Z,\Tilde{V},\hat{X}} \cdot p_{Z|X=\hat{X}} \mapsto \Tilde{p}_{X,Z,\Tilde{V},\hat{X}} 
    %\mapsto \Tilde{p}_{X,Z,\hat{X}}.
\end{equation*}This results in a map from $\Tilde{\mathcal{D}}_D$ to $\mathcal{D}_{E\text{-}D}.$ Indeed the first map makes the Markov chain in $\Tilde{\mathcal{D}}_D$ equivalent to $X - (Z, V) - \hat{X}$ and the second removes the unused variable $\hat{Z}.$ Then, $\Tilde{V}$ and $\hat{X}$ can be renamed into $V$ and $Y$ respectively.

\subsubsection{Regarding Markov chains in the converse proof}\label{app:Markov_chains_precise_reference_for_converse}
\hfill\\
In \cite[Appendix~F]{2012YassaeeEtAlInteractiveCommunicationsLongVersion},with $r=1, \omega=J,\mathcal{Y}_1=\emptyset,Y_2=Y, X_1=X, X_2=Z,C_1=M,F_1=V$, the same $V$ as in Section \ref{sec:converse} is used and the same Markov chains are proved. This extends to general alphabets since the proof in \cite{2012YassaeeEtAlInteractiveCommunicationsLongVersion} is only based on the chain rule and conditional independence, without any subtractions of mutual information terms.

\subsubsection{Use of the soft covering lemma}\label{app:use_of_soft_covering}

\begin{lemma}\label{lemma:soft_covering}\cite[Corollary~VII.4]{2013PaulCuffDistributedChannelSynthesis} Let $\mathcal{V}$ be an alphabet and $\rho_V$ a distribution on the latter. Let $R$ be a positive real number. Let $(k_n)_{n \geq 1}$ be a sequence of positive integers such that $k_n$ $\substack{\raisebox{-4pt}{$\sim$} \\ \scalebox{0.5}{$n$$\to$$\infty$}}$ $2^{n(R+\varepsilon)}.$ For every positive integer $n$ let $\mathcal{E}^{(n)}$ be a randomly generated collection of $k_n$ mutually independent sequences in $\mathcal{V}^n$ each drawn according to $\rho_V^{\otimes n}.$ The sequences are indexed by some set $\mathcal{I}$ of size $k_n$ and in a realization $e^{(n)}$ of $\mathcal{E}^{(n)}$ the sequence with index $i$ is denoted by $v^n(e^{(n)}, i).$ A memoryless channel $(\rho_{W|V\text{=}v})_{v \in \mathcal{V}}$ induces an output distribution defined as
    $$\text{$\Gamma$}\substack{\; \; \scalebox{0.85}{$(i,v^n,w^n) \qquad $} \\ \scalebox{0.6}{$I, V^n, W^n |\mathcal{E}^{(n)}=e^{(n)}$}}  = \dfrac{1}{k_n} \; \; \substack{\scalebox{1.2}{$\mathbf{1} \qquad \qquad $} \\ v^n = v^n(e^{(n)}, i)} \prod_{t=1}^n \rho \substack{\scalebox{0.8}{$ (w_t) $} \\ \scalebox{0.55}{$W|V=v_t$} } \ .$$
    If $R > I_{\rho}(V;W)$ then
    $$\mathbb{E}_{\mathcal{E}^{(n)}}\big[\|\Gamma_{W^n|\mathcal{E}^{(n)}} - \rho_{W}^{\otimes n}\|_{TV}\big] \underset{n \to \infty}{\longrightarrow} 0,$$
    \hfill\\
    where $\rho_W$ is the marginal of $\rho_{V,W} = \rho_V \cdot \rho_{W|V}.$
\end{lemma}
\hfill\\
We first use Lemma \ref{lemma:soft_covering} with $\rho = p,$ $\mathcal{E}^{(n)}=\mathcal{C}^{(n)},$ $k_n = \lfloor 2^{n(R+\varepsilon)}\rfloor \times \lfloor 2^{nR'}\rfloor \times \lfloor 2^{nR_c}\rfloor,$ $I=(M,M',J),$ $W^n=Y^n$ and $R$ replaced by $R+\varepsilon+R'+R_c.$ The corresponding output distribution is exactly $Q^{(1)}_{M,M',J, V^n, Y^n |\mathcal{C}^{(n)}= \cdot}$ thus by \eqref{eq:sum_rate_large_enough_for_Y} and Lemma \ref{lemma:soft_covering} together with the perception property $p_Y \equiv p_X$ from \eqref{eq:def_D_D} we get \eqref{eq:TV_Q_1_Y}.

Second, we use Lemma \ref{lemma:soft_covering} as follows. We fix a positive integer $j.$ For every $n$ such that $2^{nR_c}\geq j$ we set $\mathcal{E}^{(n)}$ to be the sub-codebook of $\mathcal{C}^{(n)}$ corresponding to $j$ and set $\rho = p,$ $k_n = \lfloor 2^{n(R+\varepsilon)}\rfloor \times \lfloor 2^{nR'}\rfloor.$ We further set $I=(M,M',j),$ $W=(X,Z)$ and replace $R$ in the lemma by $R+\varepsilon+R'.$ The corresponding output distribution is exactly $Q^{(1)}_{M,M', V^n, X^n, Z^n |\mathcal{C}^{(n)}= \cdot, J=j}$ thus by \eqref{eq:sum_rate_large_enough_for_X_and_Z} and Lemma \ref{lemma:soft_covering} we have
\begin{equation}\label{eq:TV_Q_1_X_Z}
    \forall j, \quad \mathbb{E}_{\mathcal{C}^{(n)}}\big[\|Q^{(1)}_{X^n, 
Z^n|\mathcal{C}^{(n)}, J=j} - p_{X, Z}^{\otimes n}\|_{TV}\big] \underset{n \to \infty}{\longrightarrow} 0.
\end{equation}

Moreover, since $Q^{(1)}_{\mathcal{C}^{(n)}, J} \equiv \mathbb{Q}_{\mathcal{C}^{(n)}}p^{\mathcal{U}}_{[2^{nR_c}]},$ then by Lemma \ref{lemma:get_expectation_out_of_TV} the total variation distance between
$Q^{(1)}_{\mathcal{C}^{(n)}, J, X^n, Z^n}$ and $\mathbb{Q}_{\mathcal{C}^{(n)}}p^{\mathcal{U}}_{[2^{nR_c}]}p_{X, Z}^{\otimes n}$ rewrites as
% \begin{IEEEeqnarray}{c}
% \mathbb{E}_{\mathcal{C}^{(n)}}\big[\|Q^{(1)}_{J, X^n, Z^n|\mathcal{C}^{(n)}} - p^{\mathcal{U}}_{[2^{nR_c}]}p_{X, Z}^{\otimes n}\|_{TV}\big]\nonumber
% \end{IEEEeqnarray}
\begin{IEEEeqnarray}{c}
    \sum_{j=1}^{\lfloor 2^{nR_c} \rfloor} \tfrac{\text{\normalsize 1}}{\lfloor 2^{nR_c} \rfloor} \mathbb{E}_{\mathcal{C}^{(n)}}\big[\|Q^{(1)}_{X^n, Z^n|\mathcal{C}^{(n)}, J=j} - p_{X, Z}^{\otimes n}\|_{TV}\big]. \nonumber
\end{IEEEeqnarray}
Finally, by construction of $\mathcal{C}^{(n)}$ the distribution of sub-codebooks $(V^n(\mathcal{C}^{(n)}, m,m',j))_{m,m'}$ is independent of $j.$ Hence all expectations in the above sum are identical. Using \eqref{eq:TV_Q_1_X_Z} we get \eqref{eq:TV_Q_1_J_X_Z}.

\subsubsection{Computations in the Gaussian case}\label{app:Gaussian}
% \subsubsection{Conditional mutual information computations in the converse proof}
\hfill\\
%\todo[inline]{In the converse, the definitions of Wyner are enough since I do not do any subtractions of mutual information terms and to deal with going from $t$ to $T$ I can do it for any discrete approximation.}
%\todo[inline]{Uniform integrability of Gaussian}
Since $\rho \geq \eta,$ we can choose
\begin{equation}\label{eq:def_b}
    b= \sqrt{(\rho^2 - \eta^2)/(1+\eta^2\rho^2-2\eta^2)}.
\end{equation}
We have $(X,Z) \sim p_{X,Z},$ the chain $Z-X-V$ and $I(Z;V) \leq h(Z) <\infty.$ By \eqref{eq:def_Z_X_V}, vector $(Z,X,V)$ is Gaussian and therefore
Then $Y$ is has normal distribution, which by \eqref{eq:rho_carre} is $\mathcal{N}(0,1) \equiv p_X$ and we have $X-(Z,V)-Y.$ 
\begin{lemma}
Let $(\Vec{x}_1, \Vec{x}_2)$ be a Gaussian vector with mean $(\Vec{\mu}_1, \Vec{\mu}_2)$ and covariance matrix \begin{equation*}
    \scalebox{0.9}{$\begin{pmatrix}
\Sigma_{11} & \Sigma_{12} \\
\Sigma_{21} & \Sigma_{12}
\end{pmatrix}$}
\end{equation*} Then, conditioned on $\Vec{x}_2\text{=}\Vec{a},$ variable $\Vec{x}_1$ is Gaussian with:
\begin{IEEEeqnarray}{c}
    \overline{\mu}_{|\Vec{a}} = \Vec{\mu}_1 + \Sigma_{12}\Sigma_{22}^{-1}(\Vec{a}-\Vec{\mu}_2)\label{eq:formula_conditiona_mean}\\
    \overline{\Sigma} = \Sigma_{11} - \Sigma_{12}\Sigma_{22}^{-1}\Sigma_{21},\label{eq:formula_conditiona_variance}
\end{IEEEeqnarray} with the covariance matrix $\overline{\Sigma}$ not depending on $\Vec{a}.$
\end{lemma}
For the centered Gaussian vector $(Z,X,V),$ we get
\begin{IEEEeqnarray}{c}
\text{Var}(X|Z) = 1 - \eta \cdot 1 \cdot \eta = 1-\eta^2 \text{ and}\label{eq:proved_Gaussian_Var_X_knowing_Z}\\
\mathbb{E}[X|Z,V]= 0 + \scalebox{0.9}{$\begin{pmatrix}
\eta & b
\end{pmatrix}$} \scalebox{0.9}{$\begin{pmatrix}
\tfrac{1}{1-\eta^2b^2} & \tfrac{-\eta b}{1-\eta^2b^2} \\
\tfrac{-\eta b}{1-\eta^2b^2} & \tfrac{1}{1-\eta^2b^2}
\end{pmatrix}$} \scalebox{0.9}{$\begin{pmatrix}
Z \\
V
\end{pmatrix}$}.\label{eq:gaussian_proof_conditional_mean}
%\\*
%&=& \dfrac{\eta-\eta b^2}{1-\eta^2 b^2}Z + \dfrac{b-\eta^2 b}{1-\eta^2 b^2}V.\label{eq:gaussian_proof_conditional_mean}
% \text{Var}[X|Z,V]= 1 - \scalebox{0.9}{$\begin{pmatrix}
% \eta & b
% \end{pmatrix}$} \scalebox{0.9}{$\begin{pmatrix}
% \tfrac{1}{1-\eta^2b^2} & \tfrac{-\eta b}{1-\eta^2b^2} \\
% \tfrac{-\eta b}{1-\eta^2b^2} & \tfrac{1}{1-\eta^2b^2}
% \end{pmatrix}$} \scalebox{0.9}{$\begin{pmatrix}
% \eta \\
% b
% \end{pmatrix}$} 
\end{IEEEeqnarray}
% \begin{IEEEeqnarray}{c}
%     \forall z, \text{Var}(X|Z=z) = 1-\eta^2 \text{ and}\label{eq:gaussian_Var_X_knowing_Z}\\*
%     \mathbb{E}[X|Z=z,V=v] = \dfrac{\eta-\eta b^2}{1-\eta^2 b^2}z + \dfrac{b-\eta^2 b}{1-\eta^2 b^2}v.\label{eq:conditional_expect_X_knowing_Z_V}
% \end{IEEEeqnarray}
%From \eqref{eq:def_Z_X_V}, \eqref{eq:def_b} and \eqref{eq:conditional_expect_X_knowing_Z_V}
%which prove \eqref{eq:gaussian_Var_X_knowing_Z} and \eqref{eq:conditional_expect_X_knowing_Z_V}. 
By \eqref{eq:def_Z_X_V}, $\mathbb{E}[Z^2]\text{=}\mathbb{E}[V^2]\text{=}1$ and $\mathbb{E}[ZV]\text{=}\eta b.$ Therefore, by \eqref{eq:gaussian_proof_conditional_mean} we have $\mathbb{E}[ \mathbb{E}[X|Z,V]^2]$
\begin{IEEEeqnarray}{rCl}
    &=& \dfrac{1}{(1\text{-}\eta^2 b^2)^2} \mathbb{E}\big[ [\eta(1\text{-}b^2)Z + b(1\text{-}\eta^2)V]^2 \big] \nonumber \\*
    &=& \dfrac{1}{(1\text{-}\eta^2 b^2)^2} \mathbb{E}\big[ \eta^2(1\text{-}b^2)^2 \text{+} b^2(1\text{-}\eta^2)^2 \text{+} 2\eta^2 b^2 (1\text{-}\eta^2)(1\text{-}b^2) \big]\IEEEeqnarraynumspace\label{eq:gaussian_developper_carre_rho_2}
\end{IEEEeqnarray}
Define $\lambda\text{=}1\text{-}\eta^2$ and $\tilde{\rho}\text{=}1-\rho^2.$ Then we have
\begin{IEEEeqnarray}{c}
    (1\text{+}\eta^2\rho^2\text{-}2\eta^2)b^2\text{=}\lambda\text{-}\tilde{\rho}, (1\text{+}\eta^2\rho^2\text{-}2\eta^2)(1\text{-}b^2)\text{=}\tilde{\rho}\lambda, \nonumber\\*
    (1\text{+}\eta^2\rho^2\text{-}2\eta^2)(1\text{-}\eta^2b^2)\text{=}\lambda^2, 1\text{+}\eta^2\rho^2\text{-}2\eta^2\text{=}\text{-}\tilde{\rho}\text{+}\lambda(1\text{+}\tilde{\rho}).\nonumber
\end{IEEEeqnarray}
Therefore, by multiplying numerator and denominator by $(1\text{+}\eta^2\rho^2\text{-}2\eta^2)^2$ in \eqref{eq:gaussian_developper_carre_rho_2} we get $\mathbb{E}[ \mathbb{E}[X|Z,V]^2]$
\begin{IEEEeqnarray}{rCl}
    &=& \dfrac{1}{\lambda^4}\Big[(1\text{-}\lambda)\tilde{\rho}^2\lambda^2\text{+}(\lambda\text{-}\tilde{\rho})\big[\text{-}\tilde{\rho}\text{+}\lambda(1\text{+}\tilde{\rho})\big]\lambda^2\text{+}2(1\text{-}\lambda)(\lambda\text{-}\tilde{\rho})\lambda\tilde{\rho}\lambda\Big] \nonumber \\*
    %&=& \scalebox{0.8}{$(1/\lambda^2)$}\Big[(1\text{-}\lambda)\tilde{\rho}^2\text{+}(\lambda\text{-}\tilde{\rho})\big[\text{-}\tilde{\rho}\text{+}\lambda(1\text{+}\tilde{\rho})\big]\text{+}2(1\text{-}\lambda)(\lambda\text{-}\tilde{\rho})\tilde{\rho}\Big]\nonumber\\*
    &=& \dfrac{1}{\lambda^2}\Big[(1\text{-}\lambda)\tilde{\rho}^2\text{+}\big[\tilde{\rho}^2\text{-}\lambda\tilde{\rho}(2\text{+}\tilde{\rho})\text{+}\lambda^2(1\text{+}\tilde{\rho})\big]\text{+}2\tilde{\rho}\big[\text{-}\tilde{\rho}\text{+}(1\text{+}\tilde{\rho})\lambda\text{-}\lambda^2\big]\Big]\nonumber\\*
    &=& \dfrac{1}{\lambda^2}\Big[1\cdot(\tilde{\rho}^2 \text{+} \tilde{\rho}^2 \text{-} 2\tilde{\rho}^2)+\lambda \cdot \big[\text{-}\tilde{\rho}^2\text{-}\tilde{\rho}(2\text{+}\tilde{\rho})\text{+}2\tilde{\rho}(1\text{+}\tilde{\rho})\big]\nonumber\\*
    &&\qquad \quad +\lambda^2\cdot\big[1\text{+}\tilde{\rho}\text{-}2\tilde{\rho}\big]\Big] \; = \tilde{\rho} = \rho^2.\nonumber
\end{IEEEeqnarray}
Finally, we compute $I(X;V|Z)$ and $\mathbb{E}[d(X,Y)].$ By translation invariance of differential entropy we have \begin{equation*}
    h(X|Z,V) = h\big(X\text{-}\mathbb{E}[X|Z,V]\big|Z,V\big).
\end{equation*}Since uncorrelated Gaussian vectors are independent, we get $h(X|Z,V) = h(X\text{-}\mathbb{E}[X|Z,V]).$ Since $\mathbb{E}[X^2]=1$ we get \begin{equation*}
    \text{Var}\big(X\text{-}\mathbb{E}[X|Z,V]\big) = 1 - \mathbb{E}[ \mathbb{E}[X|Z,V]^2].
\end{equation*}We then conclude the computation by \eqref{eq:proved_Gaussian_Var_X_knowing_Z} and \eqref{eq:rho_carre}. Also,
\begin{IEEEeqnarray}{rCl}
    \mathbb{E}[d(X,Y)] &=& \mathbb{E}[(X-\rho^{-1}\mathbb{E}[X|Z,V])^2] \nonumber \\*
    &=& 1 - 2\rho^{-1}\mathbb{E}\big[ \mathbb{E}[X|Z,V]^2 \big] + \rho^{-2}\mathbb{E}\big[ \mathbb{E}[X|Z,V]^2 \big] \nonumber \\*
    &=& 1-2\rho+1\nonumber\\*
    &=& \Delta.\label{eq:distortion_is_Delta}
\end{IEEEeqnarray}
The uniform integrability of $(d,p_X)$ is proved in \cite{2022AaronWagnerRDPTradeoffTheRoleOfCommonRandomness}. We recall the proof for completeness.\\
Let $X$ and $Y$ each have distribution $\mathcal{N}(m,\sigma^2)$ and $B$ be such that $\mathbb{P}(B)\leq \tau.$ Then by the Cauchy-Schwarz inequality:
\begin{IEEEeqnarray}{rCl}
    \mathbb{E}[(X-Y)^2\mathbf{1}_B] &\leq& \mathbb{E}[X^2]+\mathbb{E}[Y^2] + 2\mathbb{E}[(X\mathbf{1}_B)(Y\mathbf{1}_B)] \nonumber \\*
    &\leq& 2\sigma^2+ 2\sqrt{\mathbb{E}[X^2\mathbf{1}_B] \mathbb{E}[Y^2\mathbf{1}_B]}\nonumber \\*
    &\leq& 2\sigma^2+ 2\Big(\mathbb{E}[X^4]\mathbb{P}(B) \mathbb{E}[Y^4]\mathbb{P}(B)\Big)^{1/4}\nonumber\\*
    &\leq& 2\sigma^2+ 2\sqrt{\tau}\Big(\mathbb{E}[X^4] \mathbb{E}[Y^4]\Big)^{1/4}.\nonumber
\end{IEEEeqnarray} This concludes the proof since $\mathcal{N}(m,\sigma^2)$ has finite moments.

\todo[inline]{on the last page, the columns need to be balanced. Instructions for that purpose are given in the source file (they are commented out).}
