# Supplementary material for: The Rate-Distortion-Perception Trade-off with Side Information
Source: arXiv:2305.13116 source file (2023-05-22)
Supplement: Supplementary file 7 [file measure_theoretic_justifications.tex]

\subsection{Measure-theoretic justifications}
\subsubsection{General results}\label{app:measure_theory_general}
\hfill\\
%\todo[inline]{Say that we define conditional distributions of $p$ knowing null density values by using the dominating distribution, e.g. $p(x|v) = \mu$ if $?(v)=0.$ Need to fix a density $?$ to be able to talk about "the values $v$ for which $?(v)=0.$" and say once and for all that a consequence is that all distributions defined subsequently will similarly defined everywhere. And the latter and all densities are UNIQUELY defined.}
%\todo[inline]{Also clarify that any conditional distrib of $X^n, Y^n$ is w.r.t $\mu^n$ }
\todo[inline]{I think that uniform integrability does not depend on the underlying probability space as long as it is a standard probability space. If time, look at the commented todonote in Section \ref{app:info_theory_for_general_spaces}}
\todo[inline]{Check no assumption of existence of a density anywhere, unless it is $P<<P+Q$}
\todo[inline]{Fix quads and qquads in distributions}
A measurable space on a discrete alphabet will always be endowed with its power set $\sigma$-algebra and a product of the two measurable spaces will be implicitly endowed with the product $\sigma$-algebra. A conditional probability kernel is defined for all elements of the input alphabet (not just a.e.):
\begin{definition}
    Given any two measurable spaces $(\mathcal{W}, \mathcal{B})$ and $(\mathcal{W}', \mathcal{B}'),$ a \textit{regular channel}, also called a \textit{regular conditional or transition probability kernel} from the former to the latter is a function from $\mathcal{W}\times \mathcal{B}'$ to $[0,1]$ such that $\forall w \in \mathcal{W}, \rho(w,\cdot)$ is a probability distribution on $(\mathcal{W}', \mathcal{B}')$ and $\forall B' \in \mathcal{B}',$ $\rho(\cdot, B')$ is $\mathcal{B}$-measurable. The kernel is said to be \textit{dominated} by a $\sigma$-finite measure $\mu$ on $(\mathcal{W}', \mathcal{B}')$ if for every $w \in \mathcal{W},$ $\rho(w,\cdot)$ is. We then write $\rho \ll \mu.$
\end{definition}
\vspace{5pt}
% We follow standard practice in probability theory regarding product spaces and transition probabilities.
% Throughout this paper we implicitly rely on the following facts (see e.g. \cite{1995ProbabilityAndMeasure}). The domination of any joint distribution by a product $\sigma$-finite measures ensures the existence of conditional densities and probability kernels -this would also be true if one only assumed that the spaces are Polish. For every conditional probability considered we implicitly assume that one such kernel has been chosen. Moreover, domination and $\sigma$-finiteness are inherited in sequential definitions: for any joint distribution defined by a marginal and a transition kernel which are respectively dominated by two $\sigma$-finite measures, the joint distribution is dominated by the product measure and the latter is $\sigma$-finite.\\

We define measures sequentially by defining regular transition probabilities. This is well defined and grants the generalized Fubini theorem (see, e.g. \cite{1995ProbabilityAndMeasure}):
\begin{theorem}(Generalized Fubini theorem)\\
Consider any two measurable spaces $(\mathcal{W}, \mathcal{B})$ and $(\mathcal{W}', \mathcal{B}'),$ a probability measure $\mu$ on the former and a transition kernel $\rho(\cdot, \cdot)$ from $(\mathcal{W}, \mathcal{B})$ to $(\mathcal{W}', \mathcal{B}').$ Then there is a unique measure $Q$ on the product space $(\mathcal{W}\times\mathcal{W}', \mathcal{B}\otimes\mathcal{B}')$ with\begin{equation*}
    \forall B\in \mathcal{B}, \forall B' \in \mathcal{B}', \ Q(B\times B') = \int_B \rho(B',w) d\mu(w).
\end{equation*} Moreover, for any non-negative measurable function $\varphi,$ we have\begin{equation*}
    \int \varphi \ dQ = \int \bigg(\int \varphi \ d\rho(w, \cdot) \bigg) d\mu(w).
\end{equation*}
\end{theorem}
When given a joint distribution, such as from $\mathcal{D}_D,$ we extensively use corresponding conditional distributions, which is justified if the alphabets are Polish spaces accoring to the following theorem, sometimes referred to as Jirina's theorem.
\begin{theorem}\cite[Theorem~9.2.2]{BookWithJirinaTheorem2010}\label{theorem:jirina}
Let $\mathcal{W}$ and $\mathcal{W}'$ be Polish spaces and $\Omega=\mathcal{W}\times \mathcal{W}',$ endowed with their respective Borel $\sigma$-algebras. Let $Q$ be a probability measure on $\Omega,$ with marginal on $\mathcal{W}$ denoted by $\mu.$ Then, there exists a probability transition kernel $\rho(\cdot, \cdot)$ from $\mathcal{W}$ to $\mathcal{W}'$ such that for any non-negative measurable function $\varphi,$ we have\begin{equation*}
    \int \varphi \ dQ = \int \bigg(\int \varphi \ d\rho(w, \cdot) \bigg) d\mu(w).
\end{equation*}
Moreover, for any measurable set $B'\subset \mathcal{W}',$ the measurable map $w \mapsto \rho(w, B')$ is unique up to a $\mu$-null set.
\end{theorem}
\vspace{5pt}
The family of Polish spaces includes all discrete spaces and real vector spaces $\mathbb{R}^k,$ and any finite product of Polish spaces is a Polish space.

\subsubsection{Total variation distance for general alphabets}\label{app:TV_lemmas_for_general_alphabets}
\hfill\\
\todo[inline]{If time add a proof of Lemma \ref{lemma:TV_due_to_M_and_hatM}}
It is well known that the total variation distance between distributions $P,Q,$ defined by $\sup_{A}\{P(A)\text{-}Q(A)\},$ is equal to \begin{equation}
   \dfrac{1}{2} \int |p-q|d\mu = \int (p-q)^{+}d\mu,
\end{equation} for any common dominating $\mu$ and corresponding densities $p,q.$
We now prove Lemma \ref{lemma:get_expectation_out_of_TV}, \ref{lemma:TV_joint_to_TV_marginal} and \ref{lemma:TV_same_channel} in this order.
\begin{IEEEproof}
Fix a probability measure $\mu$ dominating both $\Pi_W \Pi_{L|W}$ and $\Pi_W \Gamma_{L|W}$ -e.g. ($\Pi_W \Pi_{L|W}+\Pi_W \Gamma_{L|W})/2$ - and denote the respective densities by $\pi$ and $\gamma.$ Since the alphabets are Polish, then by Theorem \ref{theorem:jirina}, measure $\mu$ admits a regular conditional probability kernel and satisfies the generalized Fubini property. Therefore, both laws have marginal $\Pi_W$ with density with respect to marginal $\mu_W$ given by \begin{equation*}
    \pi(w)=\gamma(w) = \int \pi(w,l) d\mu_{L|W=w}(l).
\end{equation*} Moreover, the transition kernels defined on $\{\pi(W)>0\}$ by \begin{equation*}
    \pi(w,\cdot)/\pi(w) \cdot \mu_{L|W=w}, \quad \gamma(w,l)/\gamma(w) \cdot \mu_{L|W=w}
\end{equation*}and some fixed distribution on $\{\pi(W)=0\}$ are regular and satisfy the generalized Fubini property because $\mu$ does. By the uniqueness result in Theorem \ref{theorem:jirina}, these kernels yield the same integrals on $\mathcal{W}\times \mathcal{L}$ as $\Pi_{L|W}$ and $\Gamma_{L|W}.$ The result is obtained by choosing $\varphi= (w,l)\mapsto|\pi(w,l)-\gamma(w,l)|$ in Theorem \ref{theorem:jirina}.
\end{IEEEproof}

\begin{IEEEproof}
    \begin{equation*}
        \sup_{A \subset \mathcal{W}\times\mathcal{L}}\{P(A)\text{-}Q(A)\} \geq \sup_{B \subset \mathcal{W}}\{P(B\times\mathcal{L})\text{-}Q(B\times\mathcal{L})\}.
    \end{equation*}
\end{IEEEproof}

\begin{IEEEproof}
    $\Pi$ and $\Gamma$ are dominated by the probability measure $\mu$ defined with marginal $\mu_W=(\Pi_W + \Gamma_W)/2$ and channel $\Pi_{L|W},$ and their densities are $d\Pi_W/d\mu_W$ and $d\Gamma_W/d\mu_W.$
\end{IEEEproof}
