# Supplementary material for: The Rate-Distortion-Perception Trade-off with Side Information
Source: arXiv:2305.13116 source file (2023-05-22)
Supplement: Supplementary file 8 [file mixed_discrete_continuous_sources.tex]

\subsection{Treatment of distributions on products of discrete and continuous alphabets}

\subsubsection{Fundamental definitions and results}\label{app:info_theory_for_general_spaces}
\hfill\\
We use the following results from \cite{Wyner1978GeneralConditionalMutualInformation} and references therein. Mutual information is well-defined for general random variables without any assumption on the underlying probability space by the two equivalent definitions.
\begin{definition}\label{def:KL_mutual_info}
Let $(X,Y)$ be a couple of joint distribution $P_{X,Y}.$ Product distribution $P_X\otimes P_Y$ is then dominated by $p_{X,Y}$ and we denote its density by $p.$ We define\begin{equation}
    I(X;Y) = \int p(x,y)\log(p(x,v))dP_{X,Y}(x,y),
\end{equation}where the negative part of the integrand is integrable. The integrand is then integrable iff $I(X;Y)<\infty.$ The term $\log(p(x,v))$ is often denoted $i(x,y).$
\end{definition}
\begin{theorem}
    \begin{equation}
        I(X;Y) = \sup_{[X], [Y]} I([X];[Y]),
    \end{equation}where $[X]$ (resp. $[Y]$) denotes any image of $X$ (resp. $Y$) by a finite-valued map.
\end{theorem}
Moreover, for the mutual information of two tuples, the supremum can be restricted to quantizations of each coordinate, ie rectangular quantization grids. Conditional mutual information is defined similarly, as well as the conditional entropy of a discrete variable conditioned on general variables. All properties of mutual information from the discrete case generalize as long as no entropy of an infinite-valued variable is used, nor any substraction of mutual information terms.
\subsubsection{Form of the soft covering lemma for mixed variables}\label{app:sup_mutual_info}
\hfill\\
The result \cite[Corollary~VII.4]{2013PaulCuffDistributedChannelSynthesis} is stated with the spectral sup-mutual information:\begin{equation*}
    \overline{I}(Z;V) = \inf\{\tau: p_{Z,V}^{\otimes n} \big( (1/n) i(Z^n,V^n) > \tau\big) \to 0\},
\end{equation*}where $i$ is as in Definition \ref{def:KL_mutual_info}. But we know that $I_p(Z;V)$ is finite, which implies that $i\log(i)$ is integrable and hence the law of large numbers applies. Therefore, by additivity of $i$ for product distributions, the spectral sup-mutual information is the mutual information.

\subsubsection{Decoder for $M'$ in the case of infinite alphabets}\label{app:decoder_M_prime}
\hfill\\
By definition of $R',$ if $I_p(Z;V)=0$ then $R'=0$ and the alphabet of $M'$ is a singleton, and therefore $M'$ can be decoded perfectly for any choice of decoder. Suppose the contrary. Then, by definition of $R'$ we have $R'<I_p(Z;V).$ 
%Moreover, if each of $\mathcal{Z}$ and $\mathcal{V}$ is finite then by the standard result for discrete memoryless channels (see e.g. \cite{Cover&Thomas2006}), the decoding error can be made to vanish as stated in Section \ref{sec:Q_1}. Suppose the contrary. Then Lemma \ref{lemma:cells_with_arbitrarily_low_probability} applies: there exists a a positive integer $\kappa$ such that in the regular quantization grid of $\mathcal{Z}\times \mathcal{V}$ of parameter $\kappa,$ the $p_{Z,V}$-probability of every cell is less that $2^{-3n(R+R'+R_c)}.$ 
Since $R'<I_p(Z;V),$ then from the results mentioned in Section \ref{app:info_theory_for_general_spaces} that there exists a quantized tuple $([Z], [V])$ such that $I_p([Z]; [V]) > R'.$ 
%and having a quantization grid that is more refined than the regular grid of parameter $\kappa.$ In particular, it is such that $[V] \equiv V$ if $\mathcal{V}$ is finite. 
As depicted in Figure \ref{fig:quantization_setup}, we extend the definition of $Q^{(1)}$ from \eqref{eq:def_Q_1} by:
\begin{figure}[t!]
    \centering\includegraphics[width=0.48\textwidth]{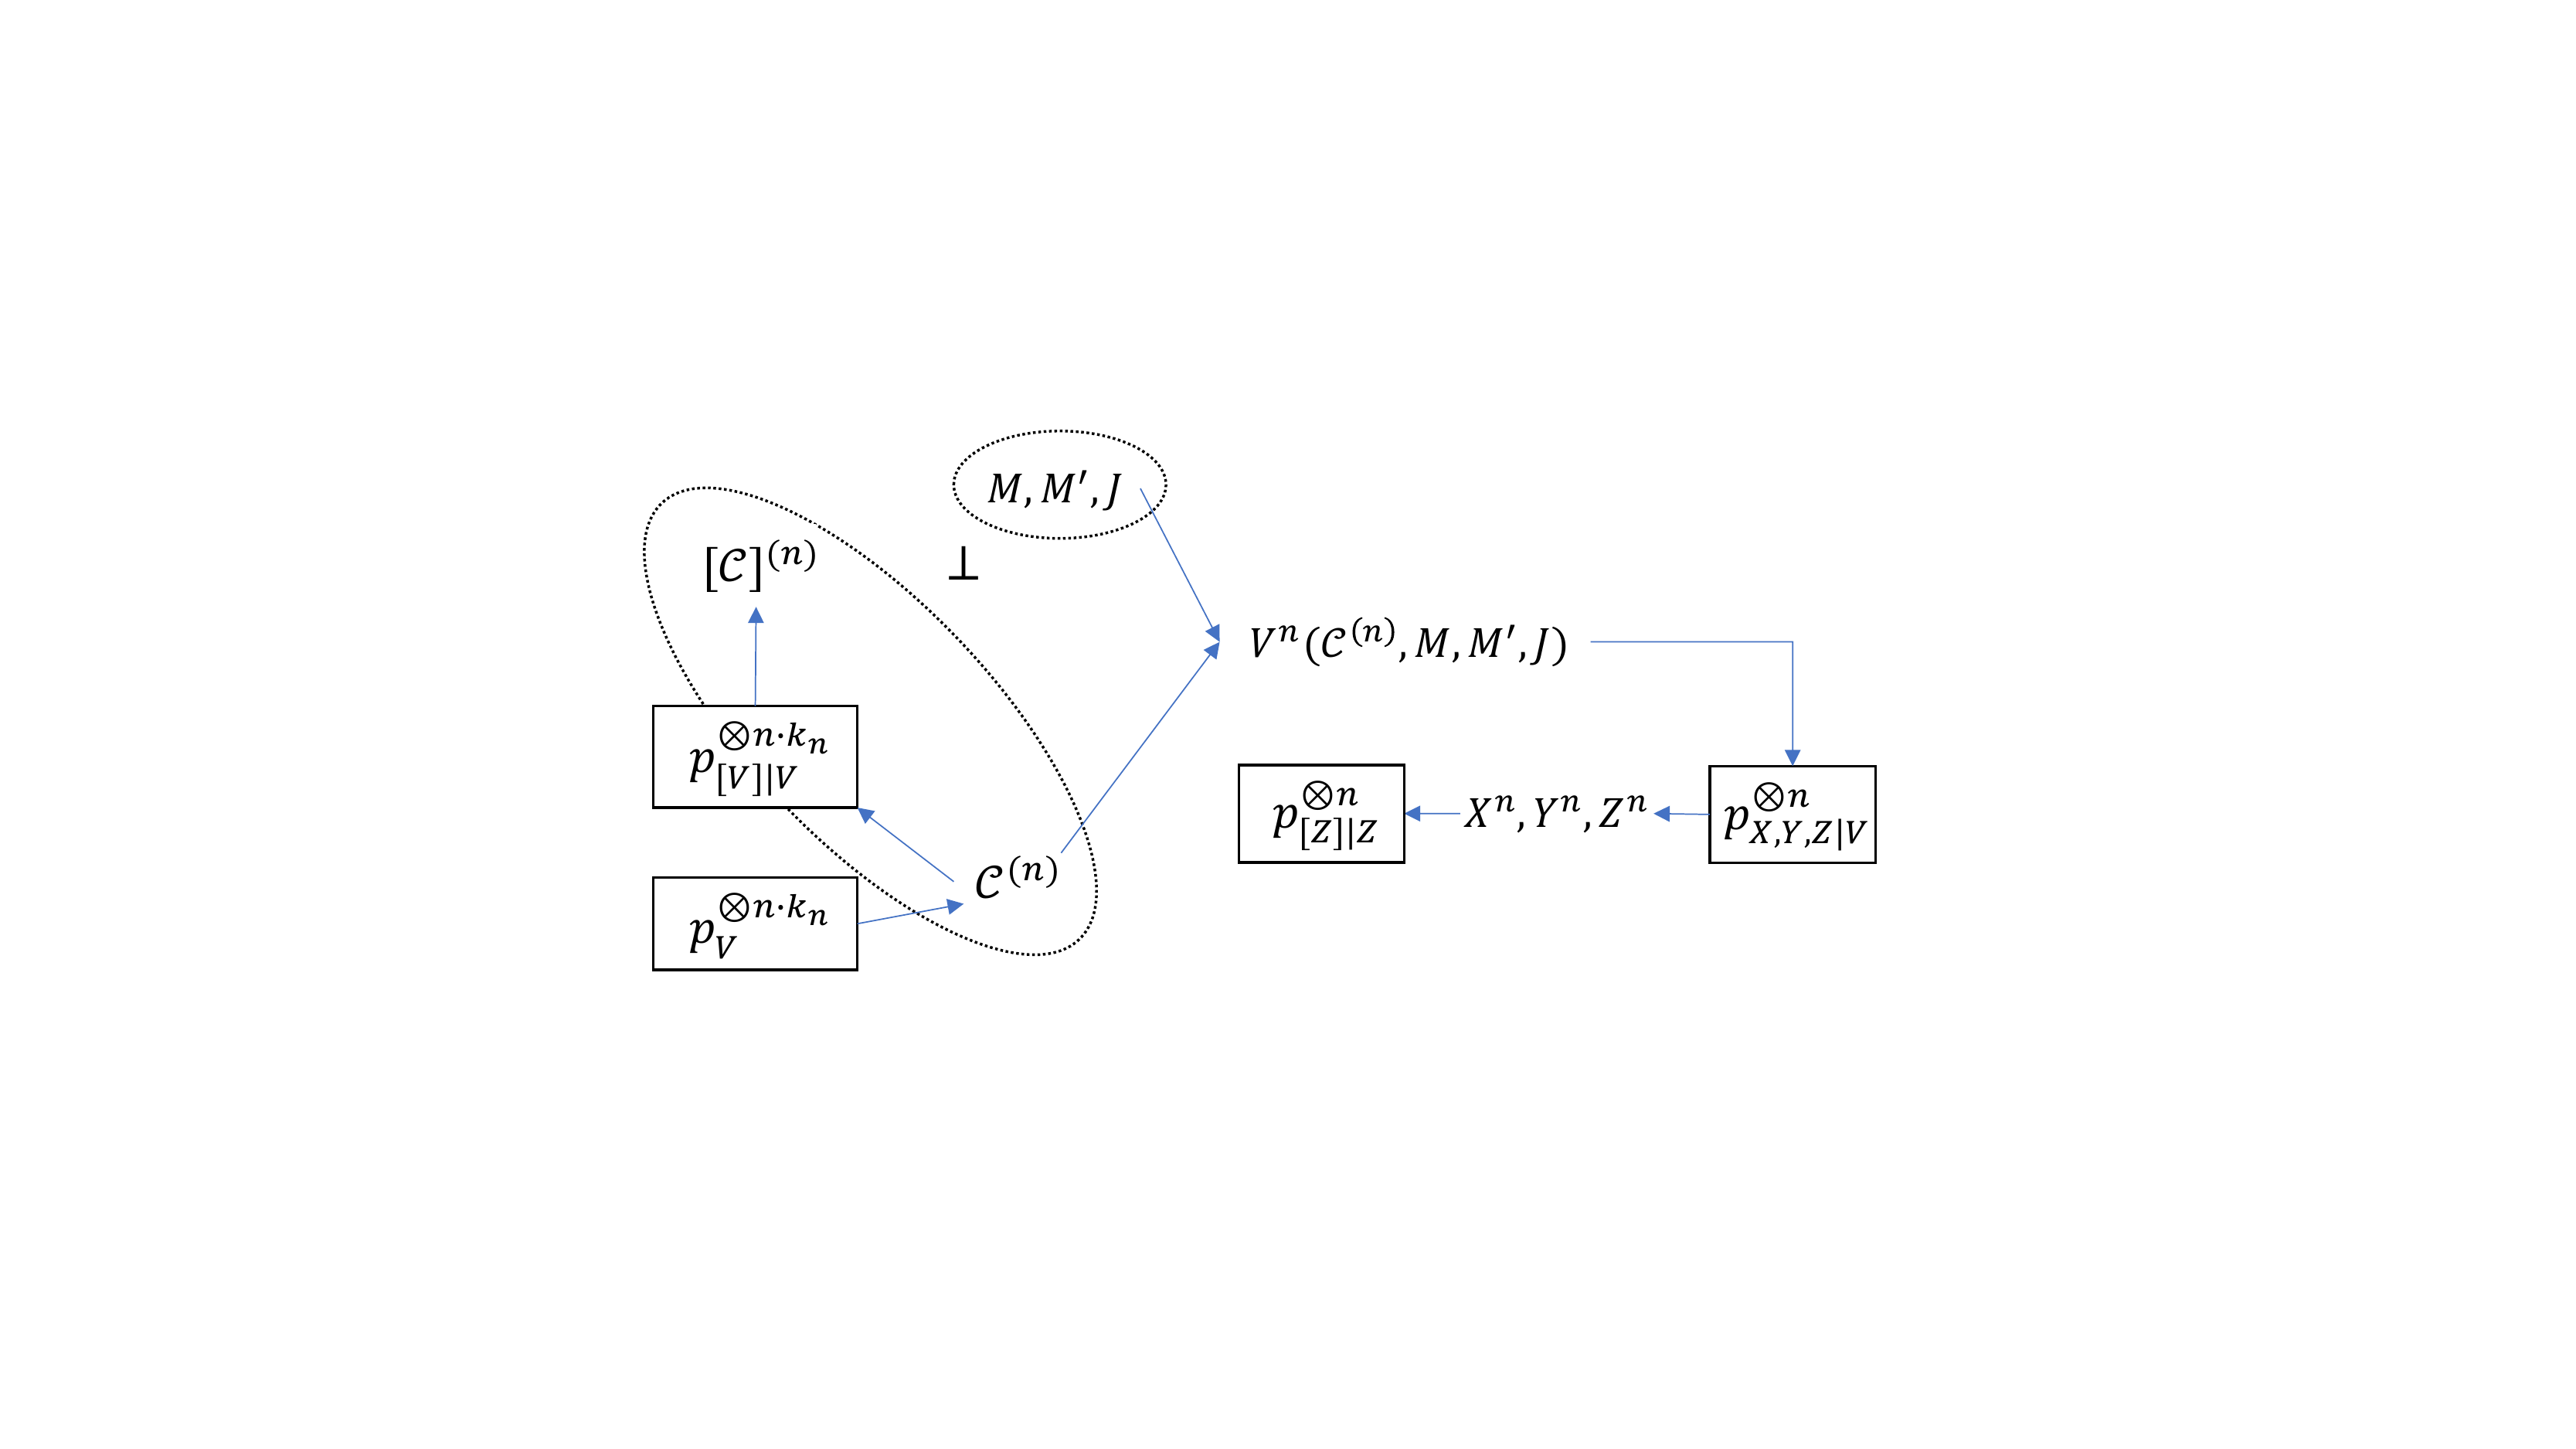}
    \caption{Graphical model for $Q^{(1)}$ with quantized variables, where $k_n = \lfloor 2^{n(R+\varepsilon)}\rfloor \times \lfloor 2^{nR'}\rfloor \times \lfloor 2^{nR_c}\rfloor.$ The variables inside a dashed oval are independent from variables inside another oval.}
    \label{fig:quantization_setup}
\end{figure}
\begin{equation}\label{eq:def_single_letter_quantization}
    p_{V,X,Y,Z,[V],[Z]} = p_{V,X,Y,Z}\cdot p_{[V]|V} \cdot p_{[Z]|Z} \text{ and}
\end{equation}\begin{IEEEeqnarray}{rCl}
\IEEEeqnarraymulticol{3}{l}{
\substack{\scalebox{1.0}{$Q^{(1)} \; ([c]^{(n)}, [z]^n, \hat{m}') \qquad \qquad \qquad \qquad \qquad \qquad \qquad \quad \;$} \\ [\mathcal{C}]^{(n)}, [Z]^n, \hat{M}' |\mathcal{C}^{(n)}\text{=}c^{(n)}, M\text{=}m, M'\text{=}m', J\text{=}j, X^n\text{=}x^n, Y^n\text{=}y^n, Z^n\text{=}z^n}
}\nonumber\\*
\quad & = & \prod_{k=1}^n \raisebox{2pt}{\scalebox{1.1}{$p$}} \substack{\scalebox{1.0}{$ \: ([z]_k)$} \\ \scalebox{0.7}{$[Z]|Z\text{=}z_k$} } \prod_{j,m,m'} \prod_{k=1}^n \raisebox{2pt}{\scalebox{1.1}{$p$}} \substack{\scalebox{1.0}{$ ([v]_k) \qquad \qquad $} \\ \scalebox{0.7}{$[V]|V\text{=}v_k(c^{(n)}, m, m', j)$} }\nonumber\\*
&& \substack{ \raisebox{-2pt}{$P^{D}$} \scalebox{1.0}{$ \; (\hat{m}') \qquad \qquad \qquad \qquad \qquad \; \ $} \\ \hat{M}' | [\mathcal{C}]^{(n)}=[c]^{(n)}, M=m, J=j, [Z]^n=[z]^n}, \label{eq:def_quantized_codebook_and_P_D}
\end{IEEEeqnarray}where $P^D$ represents, for each $(m,j),$ the joint typicality decoder of \cite{Cover&Thomas2006} for the joint distribution $p_{[V],[Z]}$ and codebook $(V^n([\mathcal{C}]^{(n)}, m, a, j))_a.$ We check that this setting is that of the channel random coding proof of \cite{Cover&Thomas2006}. Similarly to $\mathcal{C}^{(n)},$ we denote the codewords in $[\mathcal{C}]^{(n)}$ by $[V]^n([\mathcal{C}]^{(n)}, m, m', j).$\\ 

Fix a couple $(m,j).$ By the above definition \eqref{eq:def_quantized_codebook_and_P_D}, the definition of $\mathbb{Q}_{\mathcal{C}^{(n)}},$ and the independence (see \eqref{eq:def_Q_1}) of $\mathcal{C}^{(n)}$ and $(M,J)$ under $Q^{(1)},$ then knowing $M=m, J=j$ the random codebook $(V^n([\mathcal{C}]^{(n)}, j,m,a))_a$ consists of $\lfloor 2^{nR'}\rfloor$ i.i.d. codewords sampled from $p_{[V]}^{\otimes n}.$
Moreover, when conditioning on $([\mathcal{C}]^{(n)}, M,M',J)=([c]^{(n)}, m,m',j),$ as can be seen from the graphical model in Figure \ref{fig:quantization_setup} or from equations \eqref{eq:def_Q_1} and \eqref{eq:def_quantized_codebook_and_P_D}, the distribution of $[Z^n]$ is that of the output of the $n$-fold product of the discrete memoryless channel $p_{V|[V]} \cdot p_{Z|V} \cdot p_{[Z]|Z},$ with input $[v]^n([c]^{(n)}, m, m', j).$ Therefore, the proof in \cite{Cover&Thomas2006} applies: since by assumption the codebook rate satisfies $0<R'<I_p([V]; [Z]),$ we have
\begin{IEEEeqnarray}{c}
\substack{\scalebox{1.0}{$Q^{(1)} \; (\hat{M}'\neq \ M') $} \\ \hat{M}', M' |M=m, J=j } \underset{n \to \infty}{\longrightarrow} 0. \label{eq:Q_1_decoding_error_fixed_sub_codebook_general_sources} \IEEEeqnarraynumspace
\end{IEEEeqnarray}
%defining, for every $n \geq 1$ and every $(m,j) \in [2^{n(R+\varepsilon)}] \times [2^{nR_c}],$ $\Tilde{P}^{D,n}_{\hat{M}'|M, J, Z^n, \mathcal{C}^{(n)}}$ to be the joint typicality decoder applied after quantization of $Z^n,$ we get $P(\hat{M}' \neq [V^n(\mathcal{C}^n, j,m,M')]).$ Then, if $V$ is finite then by assumption the quantization is the identity map.
Since nothing in this proof depends on the particular value $(m,j),$ including the sub-codebook's distribution, the conditional distribution in \eqref{eq:Q_1_decoding_error_fixed_sub_codebook_general_sources} does not depend on $(m,j).$Hence
\begin{IEEEeqnarray}{c}
\substack{\scalebox{1.0}{$Q^{(1)} \; (\hat{M}'\neq \ M') $} \\ \hat{M}', M' \qquad \qquad} \underset{n \to \infty}{\longrightarrow} 0. \label{eq:Q_1_decoding_error_fixed_codebook_general_sources} \IEEEeqnarraynumspace
\end{IEEEeqnarray}

\todo[inline]{Replace $P_{X|Y=y}(x)$ by $P_{X|Y}(x|y)$ everywhere}
\todo[inline]{Check that no Greek letter is used for two concepts.}
